# Supplementary material for: Secure Consistency Verification for Untrusted Cloud Storage by Public Blockchains
Source: arXiv:1904.06626 source file (2019-07-29)
Supplement: Supplementary file 1 [file appendices.tex]

\section{Technical Extension on Cost Optimization}

\subsubsection{Design Alternative: On-chain storage of operations}

{\bf Use Blockchain for actual log storage}: In our protocol, all operations are uploaded to the Blockchain. An alternative design is to use the Blockchain as the actual data storage. However, Blockchain is ill-suited to be data storage serving online operations. First, Blockchain incurs multiple rounds of confirmations for persisting data, leading to perceivable write latency. Second, when operations access large data records (e.g., multimedia data), storing them directly on Blockchain incurs a high cost. Therefore, in our work, we use Blockchain as a log auditor off the critical path. It records operations at a certain frequency (e.g., every 10 minutes) and only publishes the record hashes\footnote{More precisely, given a key-value record, we can publish to the Blockchain the key hash and the value hash.} to the Blockchain.

\subsubsection{Design: Storage of Historical Operations}
For consistency verification, historical operations need to be persisted. Historical operations are those operations in the previous epochs. They are needed because an operation in the current epoch returns the record written by a historical operation.

A baseline is to maintain all historical operations on chain (e.g., in a smart-contract container). A slightly better approach is to store the ``latest'' snapshot of the records in smart contract. These baselines, however, cause high Blockchain cost as 
they directly persist data on Blockchain and Blockchain is known to be expensive for data storage.

We build a Merkle tree to enable authenticated query processing between the untrusted server and the Blockchain. Briefly, the dataset that historical operations lead to is stored on the untrusted server. The historical dataset is digested by an Merkle tree. The root hash of the Merkle tree is kept in the smart contract on chain. In an epoch, when \texttt{auditLog()} is called, the ContractChecker contract will need to query the historical dataset off-chain (see the example below). When a query of a data key is sent, an ``authentication path'' is constructed by the hash of neighbor nodes along the path from the record to the root in the Merkle tree. This authentication path can be used to prove the membership (or non-membership) of the record in the historical dataset. When \texttt{auditLog()} is completed successfully, all operations in the current epoch are reflected to the off-chain Merkle tree and the on-chain hash root is updated as well.

For instance, consider the operation sequence $w_1(K),w_2(K'),r_3[w_1](K)$ where $w_1w_2(K')$ occurs in Epoch 1 and $r_3[w_1](K)$ occur in Epoch 2. For the Blockchain to assert the consistency of $r_3[w_1]$, it will need to know as of Epoch 2 whether the latest write of data key $K$ is $w_1$. The Blockchain will send out this query to the server and the server who maintains a Merkle tree of the current state (of latest records of all data keys) returns the authentication path for $w_1$, so that its freshness can be verified by the Blockchain.

\subsubsection{Experiments: Blockchain Cost and Storage Capacity}
\begin{figure}[!hbt]
\begin{center}
\subfloat[With varying Gas cost in Ether]{
   \includegraphics[width=0.225\textwidth]{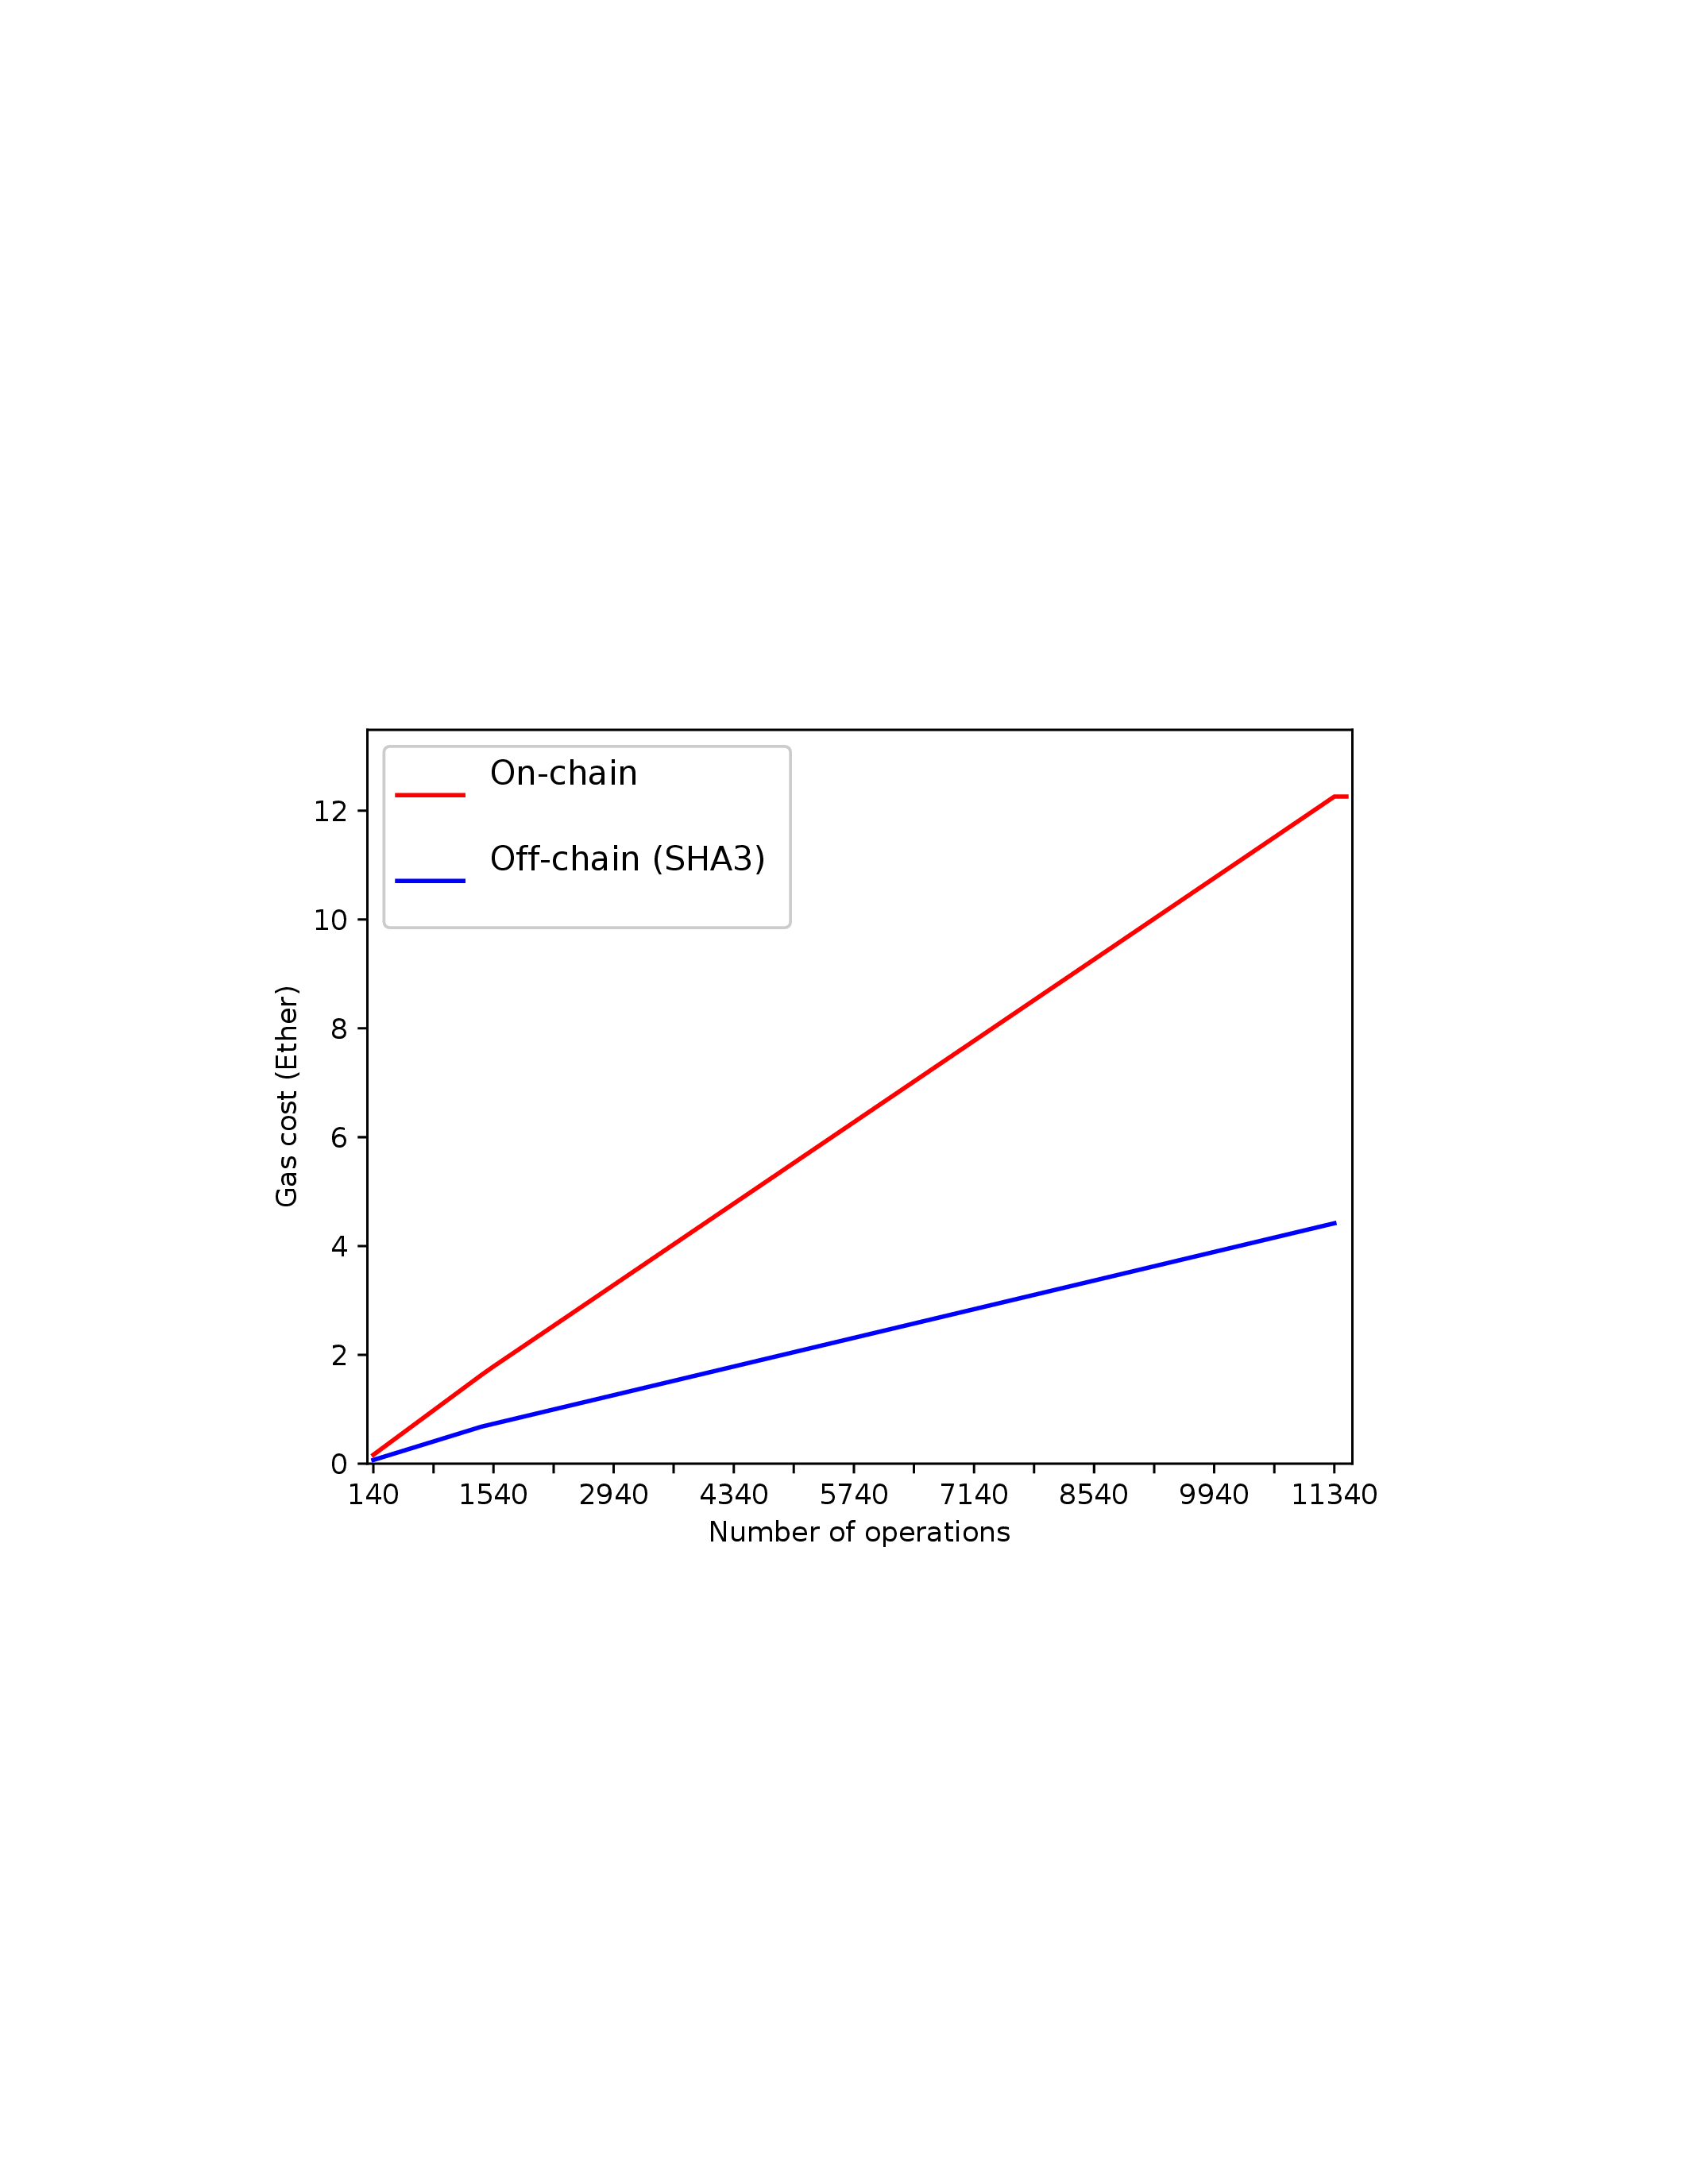}
    \label{exp:capacityether}
}
\subfloat[Storage capacity that can be bought by $\$100$]{
\includegraphics[width=0.225\textwidth]{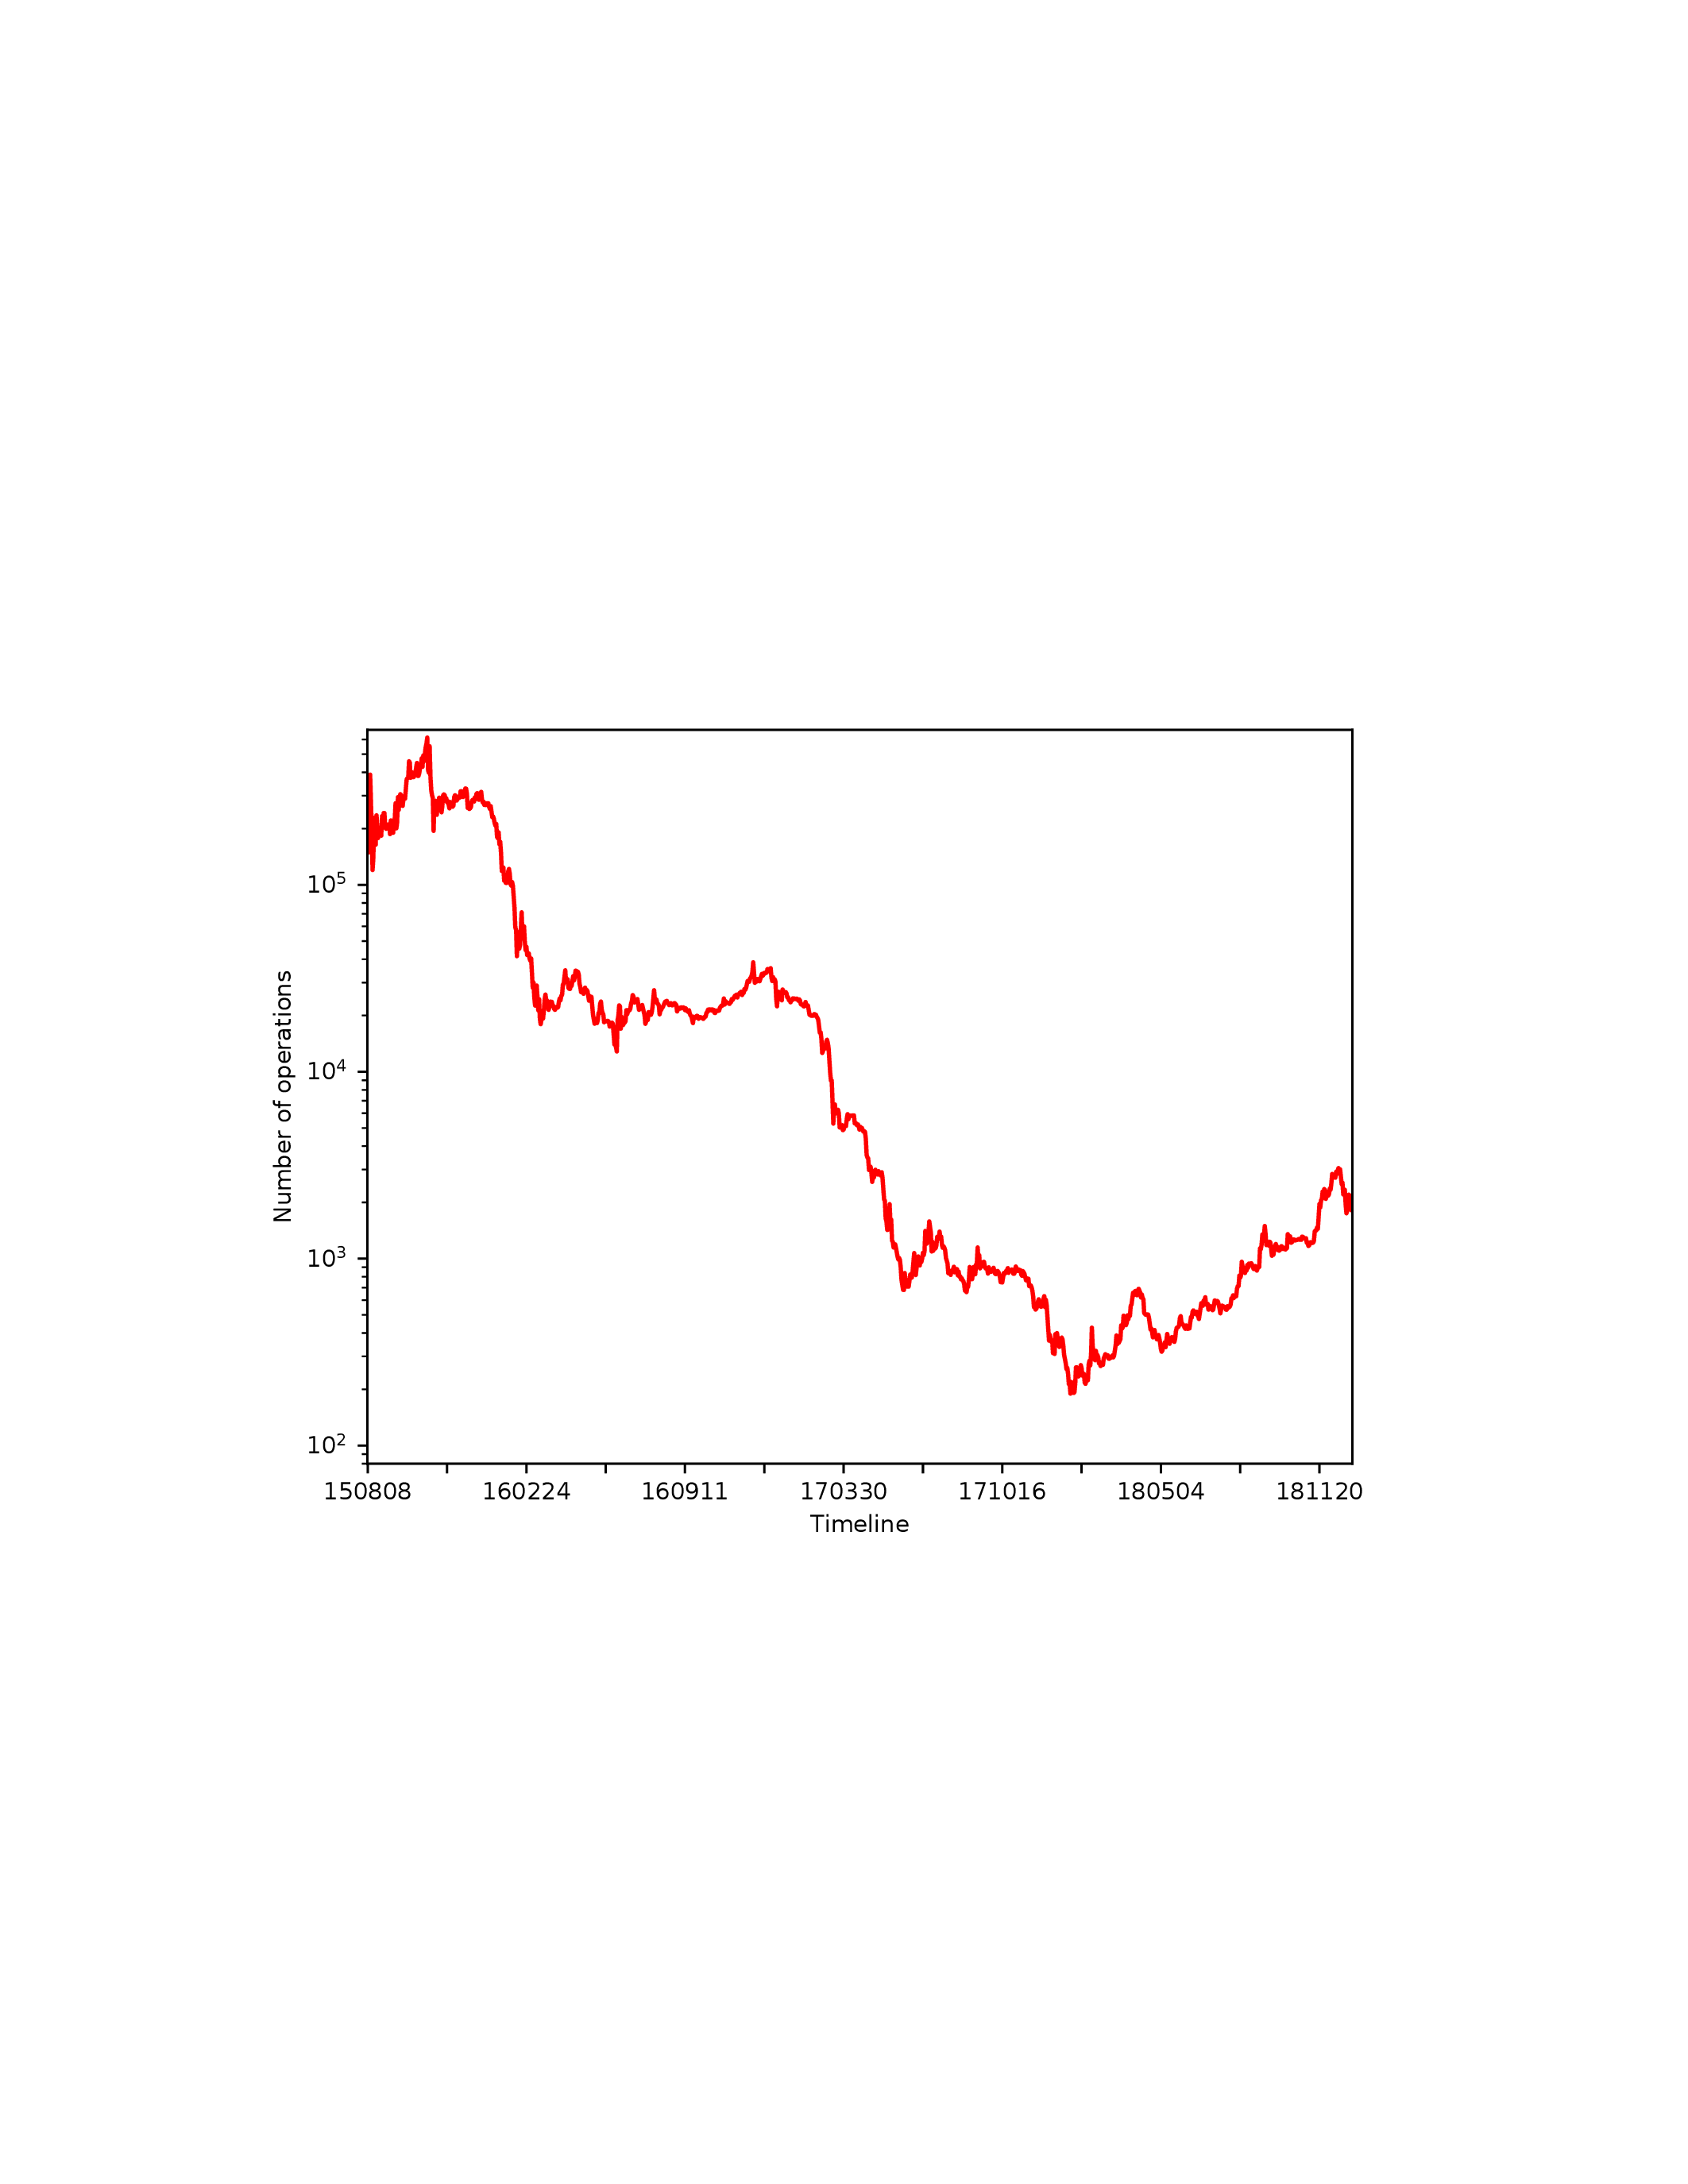}
    \label{exp:capacitydollar}
}
\end{center}
\caption{Storage capacity with Blockchain cost}
\label{exp:capacityether}
\vspace{-0.10in}
\end{figure}

This experiment measures the storage capacity with transactions fee. Given a budget of Ether, ContractChecker's storage capacity is bounded which affects the number of operations the Blockchain can consume and the maximal number of clients it can support. 

In this experiment, we use the YCSB benchmark suit. To adapt YCSB to ContractChecker, we first play and record the YCSB workload trace. We then replay the trace during the experiments. In our experiments, we set an epoch to be one block time (B) and limit 140 operations per epoch (so that Blockchain is not saturated). We set finality delay to be $F\cdot{}B = 6B$.
We drive YCSB workload D (of $95\%$ reads) into ContractChecker. The workload consists of $11340$ operations in total which are evenly distributed among $81$ epochs (with each containing $140$ operations). 
We measure the Gas cost (from the transaction receipt) with the varying number of operations. The result is in Figure~\ref{exp:capacityether}. The Gas cost grows linearly with operation count. For the off-chain placement of historical operations (of both server and client logs), the total Gas is about $4.5$ Ether for $11340$ operations. 

The off-chain placement of historical operations saves $80\%$ of the cost comparing the on-chain placement.
This result shows that transaction fee is cheaper than on-chain storage in Ethereum and the off-chain placement that trades the latter for the former is cost effective.

We also convert the Ether to US dollar and show the dollar cost with ContractChecker storage capacity. Because the price of Ether in US dollar changes over time, we present the ContractChecker storage capacity allowed by $100$ dollars at a different time. The result is illustrated in Figure~\ref{exp:capacitydollar}. It shows that with $100$ dollars, the maximal capability it can buy occurs on Oct. 2015 when the Ether is cheapest. However, as the cryptocurrency price continuously drops in 2018, the ContractChecker will be more cost-effective in US dollar.

\section{Preliminary}

\subsection{Blockchain and Smart Contract}
\label{sec:prel:bkc}

Blockchain is the backend technology in today's cryptocurrencies, such as Bitcoin and Ethereum. This work considers the public Blockchain over the Internet, and do not consider permissioned Blockchains over a private ``consortium'' of players. Physically, a public Blockchain runs in a large-scale peer-to-peer network, where peer nodes, called miners, collectively maintain Blockchain data structures. The P2P network is open-membership in that anyone on the Internet can join. 

We now present the background of Blockchain system from two perspectives that are most relevant to our work: Blockchain as a distributed ledger and Blockchain as a smart-contract execution platform.

{\bf Distributed ledger}: Blockchain is a distributed ledger that stores the history of ``transactions'' for cryptocurrency payment. The Blockchain ledger can be viewed as storage that is publicly readable and is writable by decentralized authorities namely miners. In particular, writing a transaction to Blockchain goes through the following pipeline: 1) The transaction is broadcast to all miners, pending in their memory pools. 2) Pending transactions are selected (e.g., by transaction fee) to be validated based on some prescribed rules (e.g., no double spending transactions). 3) All Blockchain nodes run a consensus protocol to decide which valid transactions are to be included next in the Blockchain ledger. Following this pipeline, every ``block time'' $B$, the Blockchain is expected to produce a new block of accepted transactions. 

Writing a transaction to a Blockchain is {\it asynchronous} in the sense that it takes a long delay to confirm if the transaction is finally included in Blockchain. More precisely, only after there are $F$ blocks produced after the transaction, the transaction is considered finalized on the Blockchain. That is, it will be hard to change the transaction state on Blockchain. Writing a transaction to a Blockchain can {\it fail} in the sense that the Blockchain can drop valid transactions in some circumstances. For example, when the transaction throughput is larger than Blockchain's throughput limits\footnote{Public Blockchains are considered as low-throughput systems that accept just tens of transactions per second.} or transaction fee is too low,  Blockchain will drop transactions. In other words, Blockchain may have low write availability in the above conditions.

{\bf Contract execution}: Blockchain is also an execution platform for \emph{smart contact}. Smart contract is a program that can be executed in modern Blockchains, such as Ethereum and that is originally proposed to support financial applications over Blockchain. To execute a smart contract, the contract author writes a program, compiles it to bytecode and deploys it to the Blockchain by encoding the compiled bytecode in a special Blockchain transaction. Once the contract is deployed on all Blockchain miners, a party off-chain will be able to trigger the contract execution by sending another transaction encoding the runtime arguments. Internally, a smart contract is executed as a replicated state machine on Blockchain miners. That is, the execution instances are spawn and replicated across all miner nodes. Running a contract function is a state transition to the Blockchain where the begin and end contract states are encoded in two blocks in Blockchain and all miners running the contract race to include the execution result in the end block.

In public Blockchain, a fundamental security assumption is that the majority of miners are honest nodes in the sense that they execute the Blockchain software by honestly following the prescribed protocol. In the case of 51\% attacks where the majority of miners are malicious, many Blockchain security properties are broken. In practice, compromising $51\%$ of miners in a large-scale Blockchain network is extremely hard and we believe this is reasonable to assume an honest majority. There are more sophisticated attacks, such as selfish mining~\cite{DBLP:conf/fc/EyalS14}, that require only $33\%$ malicious miners, but they never happen in practice and we do not consider them in this paper.

{\bf Blockchain forks}: This work focuses on practical forks in real-world public Blockchains, and excludes theoretic Blockchain forks (due to $51\%$ attacks, selfish mining, etc.). There are two types of Blockchain forks: a transient fork among miners on recently found blocks, and a permanent fork among different Blockchain networks. 
The transient fork (the former) in a public Blockchain is eventually resolved after the finality delay when all miners reach consensus on one fork while other forks are orphaned. The permanent fork (the latter) is caused by the ``hard fork'' in Blockchain software updates (e.g., the case of bitcoin and bitcoin cash), launching an Alt coin (i.e., by running Blockchain software among a group of friends), etc. It is found common in practice. 

{\bf Blockchain cost} includes the fee to send a transaction and the cost of running smart-contracts. The higher a transaction fee is, the more likely the transaction will be included in the next block. For the smart-contract, any contract on chain needs to be associated with a cost budget, called ``Gas'', which bounds the execution time of the contract and is a mechanism for the defense of DoS (denial of service) attacks.

\section{Misc. of the system}

\subsubsection{ContractChecker Epoch Configuration}
\label{sec:settinge}

ContractChecker runs in epochs. The duration of an epoch $E$ can be configured in practice to respect various application-level requirements. In general, a large $E$ is preferred when 1) the application can afford longer delay in consistency assertion, 2) the clients tend to be available in a longer time period after their interaction with the cloud server, 3) there are more clients producing more attestations transactions in an epoch.

While the first two requirements are applications specific, we present a model for the third requirement. For simplicity, we consider epoch duration $E$ is set to be multiple of the block time $B$, namely $E=e\times{}B$. 
The value of $e$ must be set large enough to avoid the attestation transactions saturate the Blockchain. For instance, suppose there are $N=30$ clients and a Block can only store 20 transactions. Setting $e=1$ may saturate the Blockchain limited throughput as every block time, the protocol produces $30+1$ transactions which are above what the Blockchain can ingest (i.e., $20$ transaction per block). In this case, it is advised to configure $e\geq{2}$, such that the $31$ attestation transactions produced in each epoch can be amortized to at least two blocks.

\subsubsection{Identity Management}
\label{sec:identity}
In ContractChecker, both clients and the server are registered in the sense that their public keys are known by the contract code. The public keys are used to verify the log attestations from clients and the server. The log verification is necessary to prevent anyone from injecting arbitrary operations in the log which can easily obstruct the consistency assertion.

To set up the public keys, we assume a secure key-distribution channel exists. Clients can dynamically join and register; we assume an external trusted identity provider in place who assists the user authentication and sends the new public keys to the smart contract.

The clients and server can reuse the public key pair in their Blockchain wallets for ContractChecker operations. In this work, we assume the secret keys are securely managed by clients and server offline. With securely managed keys, a variety of attacks, e.g., clients and server impersonation, are prevented.

\section{Motivating Applications}
\label{sec:targetapp}

%The target application scenarios of this work are cloud-hosted
%critical infrastructures. In the following we list some of the
%examples in the real world.

While ContractChecker can definitely benefit small-scale cloud-hosted
applications such as smart homes~\cite{bolt_nsdi14}, we argue that
ContractChecker can be utilized in a long spectrum of application
scenarios, ranging from low-throughput small
organizations~\cite{bolt_nsdi14}, to enterprise-scale cloud object
stores~\cite{docker_fast18}. In the following we list two representative
examples of real-world use cases. 

{\bf
DockerHub style container-distribution infrastructures} (hereafter
called ContainerRegistry):
The ``ContainerRegistry'' distributes the latest software from
developers to users in the form of Docker container images. The
ContainerRegistry is usually hosted in third-party public cloud, such
as in hub.docker.com, which is independent of both developers and
users. The storage consistency implies security as returning a stale
image (violating the strong consistency) from the hub means the users
may run buggy programs, vulnerable to the latest attacks. The
ContainerRegistry is usually accessed infrequently. For instance,
workload analysis on IBM Docker Registry reports that, among seven
geo-distributed registry deployments, the busiest one serves only 100
requests per minute for more than $80\%$ of
time~\cite{docker_fast18}\footnote{The workloads exhibit diurnal
patterns and the peak throughput is remarkably low as well.}.
%the observed throughput at IBM Docker
%Registry~\cite{docker_fast18} is
%\footnote{The workload exhibits diurnal patterns and it is the
%average load reported here.} is $100$ operations per minute.

{\bf
Certificate-transparency(CT) log}: The CT log stores the
certificates about key-identity bindings, and is made public to
invite public scrutiny for timely detection of certificate mis-issuance.
Violating storage consistency in CT log
leads to the security breaches such as concealing of mis-issued certificate or use of revoked keys.
The load of writes in a CT log (regenerating/revoking a public key) is usually low and the read load is not high on a small number of domains (websites).

{\bf
GitHub style software-development infrastructures} (hereafter
called GitHub):
GitHub provides a software-development service among collaborative developers.
The GitHub service is hosted in
the third-party public cloud and the storage consistency is security
sensitive, as exploiting inconsistency can lead to wasted
development efforts on a deserted branch~\cite{DBLP:conf/uss/Torres-AriasACC16}. The access loads in a
certain GitHub repository depend on the size of development team and
are typically not high (as commonly observed in public repositories'
committing history).

{\bf
Device synchronization thru. cloud}:
In the personal cloud services, such as Apple iCloud~\cite{icloud}, Dropbox~\cite{me:dropbox} and Microsoft OneDrive~\cite{me:onedrive},
the cloud storage is used to synchronize
multiple personal devices of the same owner.  Storage
synchronization among devices occurs at a low frequency with
remarkably low average throughput, typically once every one
hour~\cite{dropbox_imc12,mobile_cloud_imc16}. The clients are typically
low-power resource-constraint devices in this scenario. Data consistency is
important to applications where the users need to view the latest
information when switching among devices. In the real world, even though iCloud is mostly reliable, users find local updates are not synchronized fast enough, leaving a human-perceivable time to observe stale data~\cite{me:icloudsync}. Using ContractChecker presents a more proactive solution to detect the real inconsistency incidents in personal cloud services.

These application scenarios feature the following properties that motivate the use of Blockchain: 
S1) The clients are of limited capability in computing, storage, and availability. Thus they outsource data storage to a third-party cloud. In both scenarios above, the client can be a mobile phone (e.g., hosting a web browser against a CT log or installing security patches against a ContainerRegistry). 
S2) On the cloud-hosted data storage, violating storage consistency leads to a security consequence to the application. Intuitively, using a Blockchain as a ``trusted'' third-party witness can harden the application security.
S3) The storage-access load in our application scenarios is typically lower than tens of operations per second. In particular, the low throughput properties of these typical application scenarios make it amenable for the use of Blockchain, which is known to have limited throughput in ingesting transactions.

\section{Security under Client/Server Attacks}
\label{sec:clientserver:appendix}

\subsection{\bf Security against the Malicious Server}
\label{sec:servertrust}

In ContractChecker, the server's job is to declare a total-order over concurrent operations and to attest to it. A benign server is allowed to find a total-order without inconsistent operations to the degree that she does not forge operations.

Before describing the server threats, we stress that our server, be it benign or malicious, is \emph{rational}. Given a consistent operation history, a rational server does not falsely attest to a total order with inconsistency, as it does not have the incentive to do so. For instance, consider an operation history $w_1|w_2r_3[w_1]$ where $w_1$ and $w_2$ occur concurrently. A rational server will find the total-order for consistency (i.e., $w_2w_1r_3[w_1]$) and attest to it. The rational server is not incentivized to attest to the total-order with inconsistent operations (i.e., $w_1w_2r_3[w_1]$). Note that both total-orders match the real-time relation in the concurrent operation history.

{\bf Server threats}: The goal of a malicious (and rational) server is this: Given an inconsistent operation history, a malicious server aims at concealing the inconsistency by forging operations and declaring a false total order over it. In order to conceal inconsistency, the malicious server can launch a variety of threats: A malicious server forges a non-existing operation (AS1), omits the valid operation (AS2), replays a valid operation multiple times (AS3), reorders the serially-executed operations (AS4). 

{\bf Attack detection}: ContractChecker can detect the server attacks by the difference between the client logs and server log. Concretely, the server forging an operation (AS1) can be detected by an operation in the server log that cannot be found in any client log. The server omitting an operation (AS2) can be detected by an operation in a client log that cannot be found in the server log. The replay attack (AS3) can be detected by identical operations in the server log. Reordered operations (AS4) can be detected by the condition that the operation order does not match real-time (i.e., an operation that occurs later is ordered before an earlier operation). 

\subsection{\bf Security against Malicious Clients}

{\bf Client threats}: A malicious client is incentivized to falsely accuse a benign server of inconsistent operations that the server did not process. Towards this goal, a malicious client can mount the following attacks to forge her log attestation. Specifically, she omits her local operation (AC1), forges an operation the server did not process (AC2), replays a valid operation multiple times (AC3), reorder the serially-executed operations (AC4). For instance, given a consistent history, the client can forge a write operation $w_2$ between $w_1$ and $r_3[w_1]$ to make $r_3$ look like a stale read. She can omit $w_1$ to make $r_3[w_1]$ look like an invalid read. She can reorder her local operations from $w_2w_1r_3[w_1]$ to   $w_1w_2r_3[w_1]$, such that $r_3[w_1]$ is falsely inconsistent.

{\bf Attack detection}: The attacks by forging a client log can be detected by the difference between the client logs and server log. Due to no server-client collusion, we assume that the server attests to a truthful log of operations. Thus, any operation forged by the client will result in a mismatch to the server log (which can be similarly analyzed as malicious server attacks).

\subsection{\bf Security Hardening for Attack Mitigation}
\label{sec:attackmitigate}

\begin{figure}[!ht]
\begin{center}
    \includegraphics[width=0.25\textwidth]{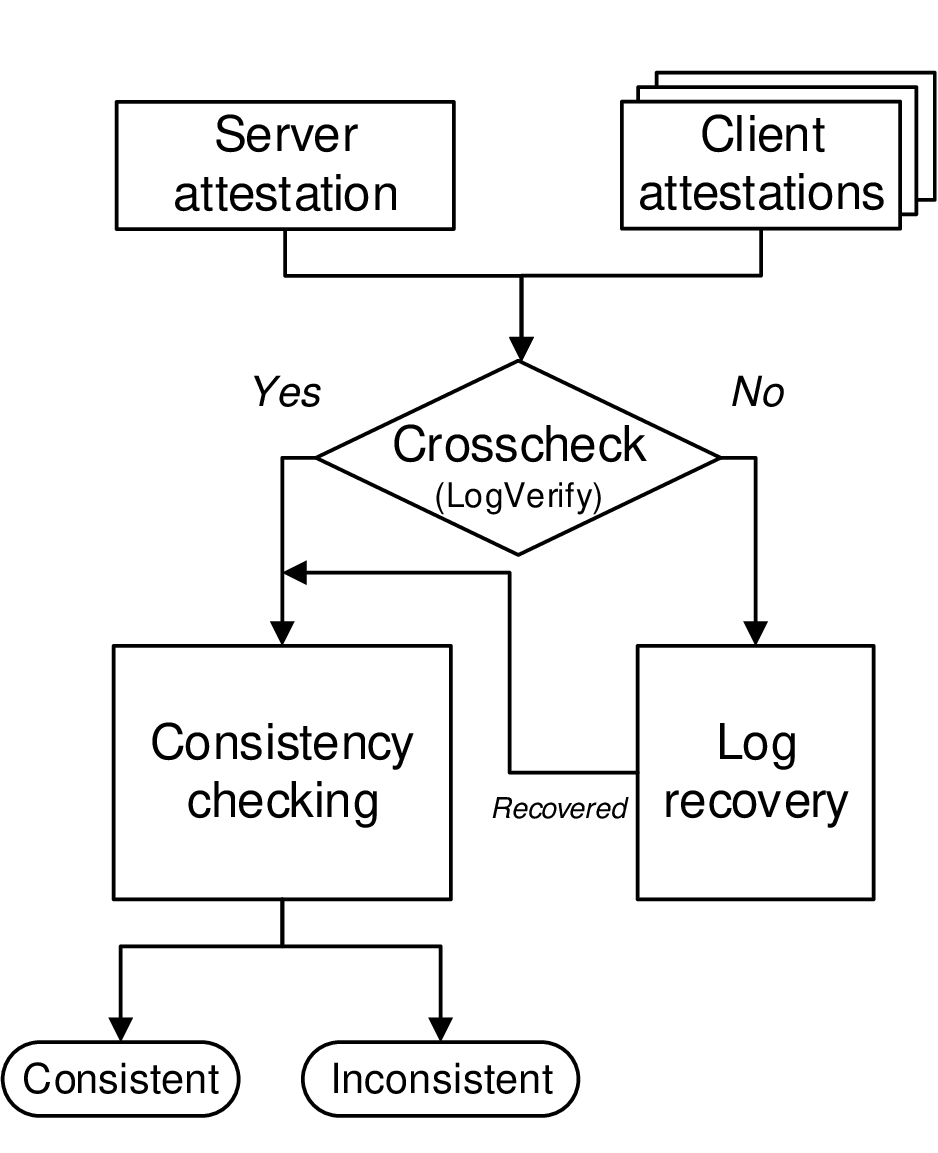}
\end{center}
%\vspace{-0.15in}
\caption{The logic in \texttt{LogAudit()} in ContractChecker for attack detection and mitigation}
\label{fig:logaudit}
\vspace{-0.10in}
\end{figure}

In the ContractChecker, attacks from a malicious server or clients are detected by the mismatch between the server attestation and client attestations (in \texttt{crosscheckLog()}). In the case of attacks, the ContractChecker does not only detect them but also mitigate them in the sense of making a trustworthy assertion about the log consistency in the presence of attacks. We describe how attacks are detected and mitigated.

In order to distinguish attacks from clients and the server, we augment the basic protocol (in \S~\ref{sec:basicprotocol}) by requiring both client and server signatures on both server attestation and client attestation. More concretely, every online operation (i.e., read/write) is augmented with a server signature and a client signature. This can be naturally integrated to the regular request/response workflow without adding extra communication round. When a client submits a request, she embeds in the request her signature of the requested operation, such that the server receives a client-signed operation. When the server processes the operation, she produces a server signature over the operation response, such that the client receives a server-signed operation response. When the client starts to do attestation, she will sign her local log of server-signed operations with the client signature. When the server starts to do attestation, she will declare the total order based on the client-signed operations. When the Blockchain receives a client attestation, it will validate the input by verifying both the client signatures and server signatures attached to the attestation. So is the case of validating a server attestation. We call this extension by double-signed attestation.

{\bf Distinguishing causes of attacks}: With the double-signed attestation, the ContractChecker can distinguish different attacks (in our threat model). When the server attestation contains an operation whose client signature cannot be verified, this is attributed to a server attack forging a non-existing operation (AS1). 
If the client signature of a server operation can be verified but the operation cannot be found in any client attestation, this is attributed to a client attack who omits her local operation (AC1). When the client attestation contains an operation whose server signature cannot be verified, it is attributed to a client attack forging an operation the server did not process (AC2). If the server signature can be verified but the operation cannot be found in the server attestation, it is attributed to a server attack omitting the operation (AS2). The replay attack (AC3 and AS3) where a client (or server) may duplicate a signed operation multiple times can be detected by finding duplicated operations on the server (or client) attestation. Normally, each operation is uniquely identified by a client-generated nonce (using an external source of trusted randomness). In addition, a malicious server (or client) may want to reorder the serially-executed operations in a different order (AC4 and AS4). This attack can be detected by the mismatch between the timestamps in the operations and the total in the attestation.

Note that we assume a rational server who will find a consistent total-order, if it exists, from the operation history and attests to it. In the case of an irrational server, she can break the protocol correctness. The irrational server can do so by intentionally declaring a total order containing inconsistent operations and by tricking the ContractChecker protocol to land a (false) assertion that the original operation history is inconsistent. To make the protocol resilient to irrational server attacks, it may require solving and declaring the total order on chain, which imposes a huge cost on the Blockchain. In addition, irrational server attacks are rare in practice. For these reasons we do not consider them in this work.

{\bf Repair server attestation}: In different attack scenarios, the ContractChecker can repair the server attestation to recover the truthful log and to further assert the log consistency. In AS1 (the server forging attack), the ContractChecker removes the forged operation from the server attestation. In AS2 (the server omission attack), the ContractChecker copy the omitted operation from the client attestation to the server attestation. In AC1 and AC2 (the client attacks by operation omission and forging), no action is needed to recover the server attestation. In replay attacks (AC3 and AS3), if it finds replayed operations on the server attestation, the ContractChecker removes the duplicated copy from the server attestation. After the repair, the ContractChecker can move forward and conduct consistency checking over the repaired server attestation. In reorder attacks (AC4 and AS4), the serial operations are reordered back to match the execution order in their timestamps.

The overall workflow of our ContractChecker for attack detection and mitigation is illustrated in Figure~\ref{fig:logaudit}.

\section{Cost-effective Security Hardening against Selective Omission Attacks}
\label{sec:costreliableatt}

To prevent the selective-omission attack, we propose a transaction-resubmission policy that provide high confidence of transaction finality within a time bound. In our policy, any active client will monitor the state of her \texttt{attestCliengLog()} call. If the finality is not confirmed after $F$ blocks, the client will increase the chance of inclusion by maximizing the transaction fee. We determine the maximal transaction fee based on heuristics in practice. High chances are that the second submission with maximal fee will make the transaction successfully included in the Blockchain.

With the resubmission policy, it can be expected all clients’ transactions in an epoch are successfully included in the Blockchain. We require that all clients wait after $2F$ blocks before using the log-consistency assertion produced by the ContractChecker program. Through this mechanism, it synchronizes across all active clients on the finality of their log attestations on Blockchain.

\section{Availability Requirement of Existing Protocols}
\label{sec:existingavailability}

{\bf Client availability in existing protocols}: In existing client-based protocols, logs are audited on the client side for checking consistency. When one client detects an attack (e.g., the server forged an operation in her log attestation), the incident needs to be reported in a timely fashion so that other clients can be notified to avoid making an incorrect assertion about log consistency.

In an untrusted server setting, the report of attack incidents is done by the untrusted server relaying messages among clients. For instance, client $c_1$ detecting an attack would send a message to the server and all other clients would pull the messages to be notified. The malicious server is able (and is well motivated) to suppress such ``attack detected’’ messages from other clients to conceal storage inconsistency. With highly available clients, this report-suppression attack itself can be detected by requiring all clients to report every epoch. Thus, the absence of a report on the server implies a report-suppression attack.

However, with unavailable clients, existing protocols relying on the untrusted server for message relay cannot guarantee protocol correctness. Be more specific, suppose a client is allowed to be offline and not to participate in the protocol in an epoch. Given the absence of the client’s report, other clients cannot distinguish between the case that the client is truly offline (the benign case) and the case that the client reports a detected attack but the malicious server suppresses it from other clients (the malicious case). Without distinguishing the two cases, other clients cannot make a correct assertion about the consistency. For instance, consider the server omits the $w_2$ in $w_1w_2r_3[w_1]$ in the attestation. If the client of $w_2$ is unavailable to audit the log in an epoch, other clients will not be aware of the omission of $w_2$ and may reach an incorrect assertion that the forged log $w_1r_3[w_1]$ seems to be consistent.

\subsection{Additional Related Work}

{\bf
Blockchain applications}: Blockchain has been applied in both financial and non-financial applications. In the application scenarios, Blockchain and its security properties are repurposed to address application-specific security needs. CSC~\cite{DBLP:journals/corr/abs-1804-05141} runs criminal smart contract on Blockchain for facilitating commissioned crimes. Paralysis~\cite{DBLP:journals/iacr/ZhangDBJ18} supports practical wallet management under key loss/compromise by using Blockchain as trusted clock to detect client unavailability. Blockstack~\cite{DBLP:conf/usenix/AliNSF16} runs trusted directory on Blockchain by treating it as immutable data storage. IKP~\cite{DBLP:conf/sp/MatsumotoR17} proposes an incentive scheme based on Blockchain to address the certificate mis-issuance problems. Blockchain is also used as the source of randomness~\cite{DBLP:books/daglib/0040621}, non-equivocation log as in Catena~\cite{DBLP:conf/sp/TomescuD17}, etc. in many novel applications.

{\bf
Blockchain throughput improvement}: There are known performance problems in Blockchain notably the limited throughput. There are protocol-analysis works on Blockchain that try to understand the throughput limitation (e.g., by block sizing~\cite{DBLP:conf/fc/CromanDEGJKMSSS16}). Lightning network~\cite{me:lightning,DBLP:journals/corr/MillerBKM17} is an off-chain scheme that batches multiple micro-payment transactions to reduce the load on chain. 
%Lightweight mining protocols are proposed including proof-of-stake~\cite{me:pos1,me:pos2}, proof-of-elapsed-time~\cite{me:poet,DBLP:conf/uss/ZhangEEJR17}, etc. Ekiden~\cite{DBLP:journals/corr/abs-1804-05141} combines Blockchain with trusted hardware to form a virtual high-throughput Blockchain system. 
Blockchain sharding~\cite{me:omniledger,DBLP:conf/ccs/LuuNZBGS16} partitions the state of transaction graph among multiple miners, in a way to improve its scalability. 

%\begin{table}[!htbp] 
%\caption{Distinction of the ContractChecker approach with existing work}
%\label{tab:distinct}\centering{\small
%\begin{tabularx}{0.5\textwidth}{ |X|c|c| }
%  \hline
%Trusted parties & Log attestation & Log auditing 
%\\ \hline
%Clients & SUNDR~\cite{DBLP:conf/osdi/LiKMS04} & Caelus~\cite{DBLP:conf/sp/KimL15}, CloudProof~\cite{DBLP:conf/usenix/PopaLMWZ11}
%\\ \hline
%Blockchain & Catena~\cite{DBLP:conf/sp/TomescuD17} & {\bf ContractChecker} (this work)
%\\ \hline
%\end{tabularx}
%}
%\end{table}

%\input{text/dsn19-appendix-11page.tex}

%%\input{text/acsac18-appendix.tex}
%\onecolumn
%see Paper_Cost folder
%\input{text_cost/icdcs19.tex}
%\newpage
%\input{text/futurework.tex}
