# Supplementary material for: Secure Consistency Verification for Untrusted Cloud Storage by Public Blockchains
Source: arXiv:1904.06626 source file (2019-07-29)
Supplement: Supplementary file 2 [file dsn19-appendix-11page.tex]

\section{ContractChecker Middleware System}
\label{sec:middleware}

The ContractChecker middleware is a distributed system that runs several jobs on individual nodes and runs remote-procedure calls (RPCs) to connect them together. Concretely, the server and clients run local logging jobs (Job 1) that log the operation histories in their respective views. The server calls a log-attestation RPC to the Blockchain by the end of each epoch (Job 2). Each client calls a log-verification RPC to the Blockchain by the end of each epoch (Job 3); This job is about the client's operation history $F$ epochs ago. The Blockchain runs log-auditing job on chain (Job 4). 
%The overall implementation of ContractChecker middleware is presented in Listing~\ref{lst:middleware}.

The local jobs such as logging (Job 1) and \texttt{auditLog} (Job 4) are implemented using native programming language. In particular, Job 4 is a smart-contract program triggered by the log-verification job. The scheduling of the jobs and events is described before in Section~\ref{sec:secureprotocols}.

Most RPCs in ContractChecker are initiated by the off-chain parties; \texttt{attestLog} is initiated by the server and \texttt{verifyLog} is initiated by individual clients. They are implemented as a smart-contract function on chain as the RPC callee and a program off-chain as the RPC caller.

\subsection{Off-chain Notification}

Some variants of ContractChecker require a reversed RPC for notification of off-chain parties. For instance, in off-chain persistent log (\S~\ref{sec:persistentlog}), the Blockchain needs to access the operations stored off-chain on server. Sending a notification from on-chain to off-chain, it presents a challenge in current Blockchain system, where transactions are sent from off-chain to on-chain. 

We implemented a basic off-chain service that virtually supports Blockchain-initiated RPCs. In this service, the Blockchain and off-chain server conceptually share a variable on-chain. The server periodically sends heartbeat messages to a smart-contract function that simply reads and returns the shared variable. The Blockchain has the write access to the shared variable. When it wants to notify the off-chain server, the Blockchain sets the value of the variable. Next time, when the server sends heartbeat transactions and calls the variable-check function, she will get a non-zero value in return. The server gets notified in a timely fashion (depending on how frequently it sends heartbeats).

\section{Client Identity Management}

In ContractChecker, clients and server are pseudo-identified by their Blockchain addresses. Their addresses are publicly known (e.g., through secure public-key distribution) and are hard-coded in the ContractChecker contract. A function in ContractChecker is associated with an intended caller. For instance, function \texttt{attestClientLog} is associated with one of clients’ addresses. When the function is called, the contract will check if the caller matches one of the intended clients.  

ContractChecker requires clients to be identified and requires each contact-function call to authenticate clients through the identity. This is necessary not only for data authenticity but also for detecting inconsistency. Without client authentication, anyone can call a ContractChecker function and inject a forged operation to the on-chain log. The forged log can violate data authenticity or consistency. For instance, the server injects a non-existing write $w_3$ between $w_1w_2$ and $r_3$; this is done by calling $\texttt{attestClientLog}(w_3)$. The forged log can accept a read returning the forged write $r_3[w_3]$, which violate data authenticity. It can also violate consistency. For instance, the server injects a non-existing delete $d_3[w_2]$ between $w_1w_2$ and $r_3[w_1]$, which can effectively conceal the inconsistency read $r_3[w_1]$ from clients.

The above, we consider the case of static membership where clients’ addresses are hard-coded in the contract. The case of dynamic membership where clients join the network can be handled by an external, trusted identity provider service which authenticates newly joined clients and update the contract with their addresses.

{\it Security}: We consider that adversaries attempt to impersonate clients and inject forged operations to the on-chain log. The adversary can do so by 1) stealing the private key of a client, and 2) updating the addresses in the contract. For the attack vector 1), we assume clients’ private keys are securely stored. In the case of stolen keys, an external mechanism exists to notify clients and contract author to revoke the address from the contract. For attack vector 2), we assume a trusted contract author and a client-authentication mechanism. An adversary cannot be authenticated as a client and a contract author will not be tricked to whitelist an adversary’s address in the contract. Note that due to the security of a digital signature, one cannot forge a signature without knowing the private signing key.

\newpage

\section{Client Identity Management (Longer)}
\subsection{Overview}
\label{sec:setup}

We consider clients are identified (e.g., by their public keys) and there is a trusted identity server who maintains a whitelist of trusted clients. During the system setup phase, each trusted client authenticates herself and register her public key with the trusted identity provider. This forms a closed membership among trusted clients. The identity provider sends the list of registered clients to the ContractChecker contract such that it can identify and authenticate clients in the online phase. The overall workflow is depicted in Figure~\ref{fig:model}. Note that the identity provider is engaged only in the system-setup phase, and is not involved in the online phase. The online-serving phase is the focus of ContractChecker protocol. 

\begin{figure}[!ht]
\begin{center}
    \includegraphics[width=0.4\textwidth]{figures/protocol1.ps}
\end{center}
%\vspace{-0.15in}
\caption{System model in ContractChecker}
\label{fig:model}
\end{figure}

\subsection{Client Identity Management: Details}
\label{sec:idp}

In ContractChecker, clients and the server are pseudo-identified by their Blockchain addresses (public keys). However, unlike a raw Blockchain, the server and clients form a closed membership network in that not everyone can join the system as a client.

For now, we consider the static membership and assume the Blockchain addresses of clients and server are hardcoded in smart contract; We will consider the dynamic client membership in Section~\ref{sec:dynmember}.

Each function call in ContractChecker performs the authentication of the caller. This is simply done by checking the equality of the RPC call's address and the hard-coded address. For instance, serving the \texttt{attestLog}, the ContractChecker authenticates the caller and checks if she is the server. Serving other calls such as \texttt{attestLog}, the ContractChecker authenticates the caller and checks if she is one of the clients. The execution of these functions proceed only when the authentication succeeds.

{\bf Client-impersonation attacks}: We consider the attack where an adversary (e.g., the untrusted server) impersonates one of the clients.\footnote{ An adversary can of course impersonate a server and send a fake log. This case can be reduced to the untrusted server in our trust mode. We don't explicitly consider this case here.} The client impersonator can validate an operation forged by the malicious server. 

Without the client authentication, client-impersonation attack can easily succeed, as anyone can call any ContractChecker function on chain and inject arbitrary data to the log. The forged log can confuse downstream computations for the consistency checking. For instance, suppose the sequence of operations is $w_1w_2r_3$. The server can forge an operation $w_3$ in sequence $w_1w_2w_3r_3$ and impersonates a client who runs \texttt{verifyLog} to validate $w_3$. The server can return $r_3[w_3]$, an incorrect result, to a genuine client. Because log $w_1w_2w_3r_3$ can be verified, this incorrect result can be detected by ContractChecker. More severely, if a delete operation is supported, the server can forge a delete operation, say $d_3[w_2]$ as in $w_1w_2d_3[w_2]r_3$, which will be validated by the impersonated client. The server can then return stale write $w_1$ as the result to the client $r_3[w_1]$, without being detected by ContractChecker.

{\bf Security analysis}: The client authentication in ContractChecker is based on public key distribution and digital signature. A client impersonator who aims at passing the authentication code on chain may need to generate a signature that can be verified by one of these public keys hard-coded (Impersonation Attack 1 or IA1). The unforgeability of digital signature~\cite{DBLP:books/crc/KatzLindell2007} ensures the client's inability to forge a signature without its private key. The impersonator can also attack by stealing the victim client's private key (IA2). We assume the private key is securely stored in each client's off-chain wallet and is not disclosed externally. The impersonator can attack by modifying the hard-coded list of client addresses and by adding its own address there (IA3). We assume the hard-coded client addresses is a read-only variable in the smart contract and we assume the memory safety of smart contract. 

\subsubsection{Dynamic Client Membership}
\label{sec:dynmember}

In this section, we address the dynamic client membership where clients can join and leave the cloud-storage system. 

The dynamic client membership is handled by an external trusted identity provider (IdP). Instead of hard-coding client membership as in the static case, the ContractChecker maintains a directory (in a mapping variable) storing the Blockchain addresses of all registered clients. During the function calls, the caller clients are authenticated using the dynamic directory of addresses. When a new client joins the system, the IdP performs its own client registration using the standard InfoSec procedure. The Blockchain address of the client is included as one of her identities. Once the registration completes, the IdP server will add the new account and her Blockchain address to the ContractChecker. When a client leaves the system, the IdP deregisters the client account and removes the Blockchain address from the ContractChecker directory.

To authenticate the IdP itself, the Blockchain address of the IdP server is static and is hard-coded in the smart contracts. 
Recall that Figure~\ref{fig:model} has shown that the Blockchain interacts the IdP server to manage identity on chain.
