# Supplementary material for: Secure Consistency Verification for Untrusted Cloud Storage by Public Blockchains
Source: arXiv:1904.06626 source file (2019-07-29)
Supplement: Supplementary file 3 [file fc19-appendix-tutorial.tex]

\section{Blockchain}

Ethereum Blockchain is a P2P network that stores valid transactions in the digital coin called Ether and executes any smart contracts written in language Solidity. Concretely, Ethereum Blockchain is an open-membership P2P network that accepts any nodes on the Internet to join as Ethereum users and/or miners. An Ethereum user who pays other users in Ether sends a transaction recording the payment to the Blockchain. Blockchain network consists of miner nodes, each of whom stores a copy of Blockchain data structure.

The purpose of Blockchain is to store the transaction history. The core data structure is a hash chain of ``blocks’’, where each block has a header that records the hash of previous block header and the Merle hash of all transactions that belong to the block. A valid block header also stores a solution to a computationally difficult puzzle.

The Blockchain runs decentralized consensus to synchronize minders’ views about the latest Blockchain in the presence of newly added transactions. The consensus runs asynchronously and it takes multiple rounds to reach a consensus on including a block. In each round, all miners race to solve a computationally difficult puzzle (i.e., proof of work) and the first one who find the solution gets to propose the next block, with rewards in Ether. The new block associated with the puzzle solution is broadcast to all other miners who will merge it with their local branch. For blocks that are deep enough, the Blockchain is fully synchronized among all miners. For blocks that are recently found, miners may have different views; that is, there are concurrent branches, the so-called accidental forks, that exist among different miners. As time goes by, among multiple concurrent branches, there will be one branch chosen and agreed by all miners, and other branches are orphaned. 

Ethereum Blockchain takes as input newly sent transactions, validates the transactions based on some predefined rules (e.g., no double-spending transactions are included), and add them to the Blockchain through mining-based consensus protocols. It is common to assume that a transaction in Blockchain is finalized only after a certain number of blocks are added.

Blockchain in this work is parameterized from two arguments: 1) the block time $B$ that is the average time a block is found in the Blockchain, and 2) the finality delay $F$ which is the number of consensus rounds needed to finalize a block on the Blockchain. 

Ethereum Blockchain supports smart contract. Conceptually the Blockchain is extended as a replicated state machine where the initial program state stored in one block is transitioned by a transaction into the end state stored in the next block. All miners in the Blockchain network faithfully execute the program and stores the result in their local chains. The smart contract is executed as an extension of transaction validation process where a validated transaction triggers the execution of contract encoded in it.
The Blockchain security provides the integrity and unstoppability of smart contract execution.

Ethereum exposes a Turing-complete programming language, called Solidity~\cite{me:sol}. 
An author writing a smart contract in Solidity deploys the contract to the Blockchain by encoding the compiled contract code in a transaction and assigning to it an address. 

{\it Blockchain forks}: A Blockchain system is subject to forks of different kinds, both theoretically and practically. In theory, a significant portion of malicious miners can collude and effectively fork the Blockchain. For instance, with $51\%$ computing power, the adversarial miners can choose a block in the past (arbitrarily deep in the Blockchain) and focus on mining on a fork. The majority of computing power makes sure the fork will eventually catch up. There are advanced mining strategies (e.g., selfish mining) that require lower mining power (e.g., $33\%$). In practice, controlling a significant portion of computing power in large Blockchain is hard. This class of forking attacks is not observed in large, deployed Blockchains, such as Bitcoin and Ethereum.
 
A Blockchain fork can be a transient fork among disconnected miners on recently found blocks. In a network of honest majority, transient forks will be eventually resolved. Be more specific, after the finality delay, there will be one transient fork that survive and all other computing forks will be orphaned. 

A Blockchain fork can also be a performant fork due to the need of updating Blockchain software and supporting Altcoin applications. This is the most ``practical’’ class of Blockchain forks. In the past, Bitcoin has been hard-forked into Bitcoin cash and Bitcoin core due to the different development plan of Bitcoin codebase. A miner can create an Altcoin by changing the transaction-validity rules on an existing Blockchain and starting to mine by herself.

Forking a Blockchain can be used to double-spend a transaction, withdraw a payment, enforce censorship, etc.

{\it Blockchain costs}: Blockchain charges transaction fees to include a transaction. There is a minimal transaction fee. Miners decide what’s in the next block based on the provided transaction fee. So a sender can increase the fee to improve the chance her transaction is included in the next block. 

Blockchain also charges ``Gas’’ when executing a smart contract. A user needs to specify the Gas budget when initiating a contract to run on Blockchain. The contract keeps execution until the Gas budget is consumed (by the miners running the contract). The unit Gas cost is defined for running different contract instructions~\cite{wood2014ethereum}. Gas prevents denial of service attacks in Blockchain.

\subsection{Preliminary}
{\it Blockchain forks}: A Blockchain system is subject to forks of different kinds, both theoretically and practically. In theory, a significant portion of malicious miners can collude and effectively fork the Blockchain. For instance, with $51\%$ computing power, the adversarial miners can choose a block in the past (arbitrarily deep in the Blockchain) and focus on mining on a fork. The majority of computing power makes sure the fork will eventually catch up. There are advanced mining strategies (e.g., selfish mining) that require lower mining power (e.g., $33\%$). In practice, controlling a significant portion of computing power in large Blockchain is hard. This class of forking attacks is not observed in large, deployed Blockchains, such as Bitcoin and Ethereum.
 
A Blockchain fork can be a transient fork among disconnected miners on recently found blocks. In a network of honest majority, transient forks will be eventually resolved. Be more specific, after the finality delay, there will be one transient fork that survive and all other computing forks will be orphaned. 

A Blockchain fork can also be a performant fork due to the need of updating Blockchain software and supporting Altcoin applications. This is the most ``practical’’ class of Blockchain forks. In the past, Bitcoin has been hard-forked into Bitcoin cash and Bitcoin core due to the different development plan of Bitcoin codebase. A miner can create an Altcoin by changing the transaction-validity rules on an existing Blockchain and starting to mine by herself.

Forking a Blockchain can be used to double-spend a transaction, withdraw a payment, enforce censorship, etc.

{\it Blockchain costs}: Blockchain charges transaction fees to include a transaction. There is a minimal transaction fee. Miners decide what’s in the next block based on the provided transaction fee. So a sender can increase the fee to improve the chance her transaction is included in the next block. 

Blockchain also charges ``Gas’’ when executing a smart contract. A user needs to specify the Gas budget when initiating a contract to run on Blockchain. The contract keeps execution until the Gas budget is consumed (by the miners running the contract). The unit Gas cost is defined for running different contract instructions~\cite{wood2014ethereum}. Gas prevents denial of service attacks in Blockchain.
