# Supplementary material for: Secure Consistency Verification for Untrusted Cloud Storage by Public Blockchains
Source: arXiv:1904.06626 source file (2019-07-29)
Supplement: Supplementary file 4 [file asiaccs19-appendix.tex]

\section{Motivating Applications}
\label{sec:targetapp}

%The target application scenarios of this work are cloud-hosted
%critical infrastructures. In the following we list some of the
%examples in the real world.

While ContractChecker can definitely benefit small-scale cloud-hosted
applications such as smart homes~\cite{bolt_nsdi14}, we argue that
ContractChecker can be utilized in a long spectrum of application
scenarios, ranging from low-throughput small
organizations~\cite{bolt_nsdi14}, to enterprise-scale cloud object
stores~\cite{docker_fast18}. In the following we list two representative
examples of real-world use cases. 

{\bf
DockerHub style container-distribution infrastructures} (hereafter
called ContainerRegistry):
The ``ContainerRegistry'' distributes the latest software from
developers to users in the form of Docker container images. The
ContainerRegistry is usually hosted in third-party public cloud, such
as in hub.docker.com, which is independent of both developers and
users. The storage consistency implies security as returning a stale
image (violating the strong consistency) from the hub means the users
may run buggy programs, vulnerable to the latest attacks. The
ContainerRegistry is usually accessed infrequently. For instance,
workload analysis on IBM Docker Registry reports that, among seven
geo-distributed registry deployments, the busiest one serves only 100
requests per minute for more than $80\%$ of
time~\cite{docker_fast18}\footnote{The workloads exhibit diurnal
patterns and the peak throughput is remarkably low as well.}.
%the observed throughput at IBM Docker
%Registry~\cite{docker_fast18} is
%\footnote{The workload exhibits diurnal patterns and it is the
%average load reported here.} is $100$ operations per minute.

{\bf
Certificate-transparency(CT) log}: The CT log stores the
certificates about key-identity bindings, and is made public to
invite public scrutiny for timely detection of certificate mis-issuance.
Violating storage consistency in CT log
leads to the security breaches such as concealing of mis-issued certificate or use of revoked keys.
The load of writes in a CT log (regenerating/revoking a public key) is usually low and the read load is not high on a small number of domains (websites).

{\bf
GitHub style software-development infrastructures} (hereafter
called GitHub):
GitHub provides a software-development service among collaborative developers.
The GitHub service is hosted in
the third-party public cloud and the storage consistency is security
sensitive, as exploiting inconsistency can lead to wasted
development efforts on a deserted branch~\cite{DBLP:conf/uss/Torres-AriasACC16}. The access loads in a
certain GitHub repository depend on the size of development team and
are typically not high (as commonly observed in public repositories'
committing history).

{\bf
Device synchronization thru. cloud}:
In the personal cloud services, such as Apple iCloud~\cite{icloud}, Dropbox~\cite{me:dropbox} and Microsoft OneDrive~\cite{me:onedrive},
the cloud storage is used to synchronize
multiple personal devices of the same owner.  Storage
synchronization among devices occurs at a low frequency with
remarkably low average throughput, typically once every one
hour~\cite{dropbox_imc12,mobile_cloud_imc16}. The clients are typically
low-power resource-constraint devices in this scenario. Data consistency is
important to applications where the users need to view the latest
information when switching among devices. In the real world, even though iCloud is mostly reliable, users find local updates are not synchronized fast enough, leaving a human-perceivable time to observe stale data~\cite{me:icloudsync}. Using ContractChecker presents a more proactive solution to detect the real inconsistency incidents in personal cloud services.

These application scenarios feature the following properties that motivate the use of Blockchain: 
S1) The clients are of limited capability in computing, storage, and availability. Thus they outsource data storage to a third-party cloud. In both scenarios above, the client can be a mobile phone (e.g., hosting a web browser against a CT log or installing security patches against a ContainerRegistry). 
S2) On the cloud-hosted data storage, violating storage consistency leads to a security consequence to the application. Intuitively, using a Blockchain as a ``trusted'' third-party witness can harden the application security.
S3) The storage-access load in our application scenarios is typically lower than tens of operations per second. In particular, the low throughput properties of these typical application scenarios make it amenable for the use of Blockchain, which is known to have limited throughput in ingesting transactions.

\section{Security under Client/Server Attacks}
\label{sec:clientserver:appendix}

\subsection{\bf Security against the Malicious Server}
\label{sec:servertrust}

In ContractChecker, the server's job is to declare a total-order over concurrent operations and to attest to it. A benign server is allowed to find a total-order without inconsistent operations to the degree that she does not forge operations.

Before describing the server threats, we stress that our server, be it benign or malicious, is \emph{rational}. Given a consistent operation history, a rational server does not falsely attest to a total order with inconsistency, as it does not have the incentive to do so. For instance, consider an operation history $w_1|w_2r_3[w_1]$ where $w_1$ and $w_2$ occur concurrently. A rational server will find the total-order for consistency (i.e., $w_2w_1r_3[w_1]$) and attest to it. The rational server is not incentivized to attest to the total-order with inconsistent operations (i.e., $w_1w_2r_3[w_1]$). Note that both total-orders match the real-time relation in the concurrent operation history.

{\bf Server threats}: The goal of a malicious (and rational) server is this: Given an inconsistent operation history, a malicious server aims at concealing the inconsistency by forging operations and declaring a false total order over it. In order to conceal inconsistency, the malicious server can launch a variety of threats: A malicious server forges a non-existing operation (AS1), omits the valid operation (AS2), replays a valid operation multiple times (AS3), reorders the serially-executed operations (AS4). 

{\bf Attack detection}: ContractChecker can detect the server attacks by the difference between the client logs and server log. Concretely, the server forging an operation (AS1) can be detected by an operation in the server log that cannot be found in any client log. The server omitting an operation (AS2) can be detected by an operation in a client log that cannot be found in the server log. The replay attack (AS3) can be detected by identical operations in the server log. Reordered operations (AS4) can be detected by the condition that the operation order does not match real-time (i.e., an operation that occurs later is ordered before an earlier operation). 

\subsection{\bf Security against Malicious Clients}

{\bf Client threats}: A malicious client is incentivized to falsely accuse a benign server of inconsistent operations that the server did not process. Towards this goal, a malicious client can mount the following attacks to forge her log attestation. Specifically, she omits her local operation (AC1), forges an operation the server did not process (AC2), replays a valid operation multiple times (AC3), reorder the serially-executed operations (AC4). For instance, given a consistent history, the client can forge a write operation $w_2$ between $w_1$ and $r_3[w_1]$ to make $r_3$ look like a stale read. She can omit $w_1$ to make $r_3[w_1]$ look like an invalid read. She can reorder her local operations from $w_2w_1r_3[w_1]$ to   $w_1w_2r_3[w_1]$, such that $r_3[w_1]$ is falsely inconsistent.

{\bf Attack detection}: The attacks by forging a client log can be detected by the difference between the client logs and server log. Due to no server-client collusion, we assume that the server attests to a truthful log of operations. Thus, any operation forged by the client will result in a mismatch to the server log (which can be similarly analyzed as malicious server attacks).

\subsection{\bf Security Hardening for Attack Mitigation}
\label{sec:attackmitigate}

\begin{figure}[!ht]
\begin{center}
    \includegraphics[width=0.25\textwidth]{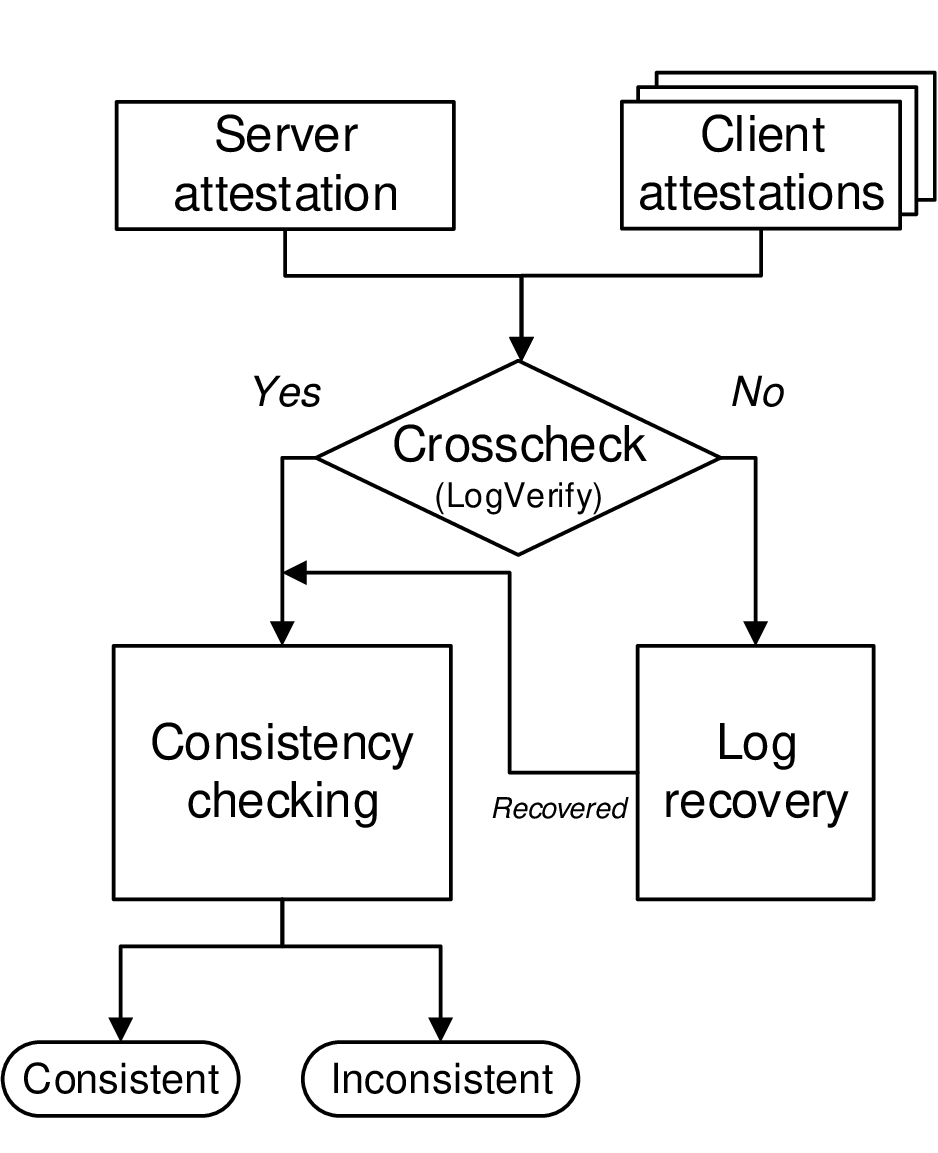}
\end{center}
%\vspace{-0.15in}
\caption{The logic in \texttt{LogAudit()} in ContractChecker for attack detection and mitigation}
\label{fig:logaudit}
\vspace{-0.10in}
\end{figure}

In the ContractChecker, attacks from a malicious server or clients are detected by the mismatch between the server attestation and client attestations (in \texttt{crosscheckLog()}). In the case of attacks, the ContractChecker does not only detect them but also mitigate them in the sense of making a trustworthy assertion about the log consistency in the presence of attacks. We describe how attacks are detected and mitigated.

In order to distinguish attacks from clients and the server, we augment the basic protocol (in \S~\ref{sec:basicprotocol}) by requiring both client and server signatures on both server attestation and client attestation. More concretely, every online operation (i.e., read/write) is augmented with a server signature and a client signature. This can be naturally integrated to the regular request/response workflow without adding extra communication round. When a client submits a request, she embeds in the request her signature of the requested operation, such that the server receives a client-signed operation. When the server processes the operation, she produces a server signature over the operation response, such that the client receives a server-signed operation response. When the client starts to do attestation, she will sign her local log of server-signed operations with the client signature. When the server starts to do attestation, she will declare the total order based on the client-signed operations. When the Blockchain receives a client attestation, it will validate the input by verifying both the client signatures and server signatures attached to the attestation. So is the case of validating a server attestation. We call this extension by double-signed attestation.

{\bf Distinguishing causes of attacks}: With the double-signed attestation, the ContractChecker can distinguish different attacks (in our threat model). When the server attestation contains an operation whose client signature cannot be verified, this is attributed to a server attack forging a non-existing operation (AS1). 
If the client signature of a server operation can be verified but the operation cannot be found in any client attestation, this is attributed to a client attack who omits her local operation (AC1). When the client attestation contains an operation whose server signature cannot be verified, it is attributed to a client attack forging an operation the server did not process (AC2). If the server signature can be verified but the operation cannot be found in the server attestation, it is attributed to a server attack omitting the operation (AS2). The replay attack (AC3 and AS3) where a client (or server) may duplicate a signed operation multiple times can be detected by finding duplicated operations on the server (or client) attestation. Normally, each operation is uniquely identified by a client-generated nonce (using an external source of trusted randomness). In addition, a malicious server (or client) may want to reorder the serially-executed operations in a different order (AC4 and AS4). This attack can be detected by the mismatch between the timestamps in the operations and the total in the attestation.

Note that we assume a rational server who will find a consistent total-order, if it exists, from the operation history and attests to it. In the case of an irrational server, she can break the protocol correctness. The irrational server can do so by intentionally declaring a total order containing inconsistent operations and by tricking the ContractChecker protocol to land a (false) assertion that the original operation history is inconsistent. To make the protocol resilient to irrational server attacks, it may require solving and declaring the total order on chain, which imposes a huge cost on the Blockchain. In addition, irrational server attacks are rare in practice. For these reasons we do not consider them in this work.

{\bf Repair server attestation}: In different attack scenarios, the ContractChecker can repair the server attestation to recover the truthful log and to further assert the log consistency. In AS1 (the server forging attack), the ContractChecker removes the forged operation from the server attestation. In AS2 (the server omission attack), the ContractChecker copy the omitted operation from the client attestation to the server attestation. In AC1 and AC2 (the client attacks by operation omission and forging), no action is needed to recover the server attestation. In replay attacks (AC3 and AS3), if it finds replayed operations on the server attestation, the ContractChecker removes the duplicated copy from the server attestation. After the repair, the ContractChecker can move forward and conduct consistency checking over the repaired server attestation. In reorder attacks (AC4 and AS4), the serial operations are reordered back to match the execution order in their timestamps.

The overall workflow of our ContractChecker for attack detection and mitigation is illustrated in Figure~\ref{fig:logaudit}.

\section{Cost-effective Security Hardening against Selective Omission Attacks}
\label{sec:costreliableatt}

To prevent the selective-omission attack, we propose a transaction-resubmission policy that provide high confidence of transaction finality within a time bound. In our policy, any active client will monitor the state of her \texttt{attestCliengLog()} call. If the finality is not confirmed after $F$ blocks, the client will increase the chance of inclusion by maximizing the transaction fee. We determine the maximal transaction fee based on heuristics in practice. High chances are that the second submission with maximal fee will make the transaction successfully included in the Blockchain.

With the resubmission policy, it can be expected all clients’ transactions in an epoch are successfully included in the Blockchain. We require that all clients wait after $2F$ blocks before using the log-consistency assertion produced by the ContractChecker program. Through this mechanism, it synchronizes across all active clients on the finality of their log attestations on Blockchain.

\section{Availability Requirement of Existing Protocols}
\label{sec:existingavailability}

{\bf Client availability in existing protocols}: In existing client-based protocols, logs are audited on the client side for checking consistency. When one client detects an attack (e.g., the server forged an operation in her log attestation), the incident needs to be reported in a timely fashion so that other clients can be notified to avoid making an incorrect assertion about log consistency.

In an untrusted server setting, the report of attack incidents is done by the untrusted server relaying messages among clients. For instance, client $c_1$ detecting an attack would send a message to the server and all other clients would pull the messages to be notified. The malicious server is able (and is well motivated) to suppress such ``attack detected’’ messages from other clients to conceal storage inconsistency. With highly available clients, this report-suppression attack itself can be detected by requiring all clients to report every epoch. Thus, the absence of a report on the server implies a report-suppression attack.

However, with unavailable clients, existing protocols relying on the untrusted server for message relay cannot guarantee protocol correctness. Be more specific, suppose a client is allowed to be offline and not to participate in the protocol in an epoch. Given the absence of the client’s report, other clients cannot distinguish between the case that the client is truly offline (the benign case) and the case that the client reports a detected attack but the malicious server suppresses it from other clients (the malicious case). Without distinguishing the two cases, other clients cannot make a correct assertion about the consistency. For instance, consider the server omits the $w_2$ in $w_1w_2r_3[w_1]$ in the attestation. If the client of $w_2$ is unavailable to audit the log in an epoch, other clients will not be aware of the omission of $w_2$ and may reach an incorrect assertion that the forged log $w_1r_3[w_1]$ seems to be consistent.

\subsection{Additional Related Work}

{\bf
Blockchain applications}: Blockchain has been applied in both financial and non-financial applications. In the application scenarios, Blockchain and its security properties are repurposed to address application-specific security needs. CSC~\cite{DBLP:journals/corr/abs-1804-05141} runs criminal smart contract on Blockchain for facilitating commissioned crimes. Paralysis~\cite{DBLP:journals/iacr/ZhangDBJ18} supports practical wallet management under key loss/compromise by using Blockchain as trusted clock to detect client unavailability. Blockstack~\cite{DBLP:conf/usenix/AliNSF16} runs trusted directory on Blockchain by treating it as immutable data storage. IKP~\cite{DBLP:conf/sp/MatsumotoR17} proposes an incentive scheme based on Blockchain to address the certificate mis-issuance problems. Blockchain is also used as the source of randomness~\cite{DBLP:books/daglib/0040621}, non-equivocation log as in Catena~\cite{DBLP:conf/sp/TomescuD17}, etc. in many novel applications.

{\bf
Blockchain throughput improvement}: There are known performance problems in Blockchain notably the limited throughput. There are protocol-analysis works on Blockchain that try to understand the throughput limitation (e.g., by block sizing~\cite{DBLP:conf/fc/CromanDEGJKMSSS16}). Lightning network~\cite{me:lightning,DBLP:journals/corr/MillerBKM17} is an off-chain scheme that batches multiple micro-payment transactions to reduce the load on chain. 
%Lightweight mining protocols are proposed including proof-of-stake~\cite{me:pos1,me:pos2}, proof-of-elapsed-time~\cite{me:poet,DBLP:conf/uss/ZhangEEJR17}, etc. Ekiden~\cite{DBLP:journals/corr/abs-1804-05141} combines Blockchain with trusted hardware to form a virtual high-throughput Blockchain system. 
Blockchain sharding~\cite{me:omniledger,DBLP:conf/ccs/LuuNZBGS16} partitions the state of transaction graph among multiple miners, in a way to improve its scalability. 

%\begin{table}[!htbp] 
%\caption{Distinction of the ContractChecker approach with existing work}
%\label{tab:distinct}\centering{\small
%\begin{tabularx}{0.5\textwidth}{ |X|c|c| }
%  \hline
%Trusted parties & Log attestation & Log auditing 
%\\ \hline
%Clients & SUNDR~\cite{DBLP:conf/osdi/LiKMS04} & Caelus~\cite{DBLP:conf/sp/KimL15}, CloudProof~\cite{DBLP:conf/usenix/PopaLMWZ11}
%\\ \hline
%Blockchain & Catena~\cite{DBLP:conf/sp/TomescuD17} & {\bf ContractChecker} (this work)
%\\ \hline
%\end{tabularx}
%}
%\end{table}
