# Supplementary material for: Secure Consistency Verification for Untrusted Cloud Storage by Public Blockchains
Source: arXiv:1904.06626 source file (2019-07-29)
Supplement: Supplementary file 5 [file securecomm19-appendix.tex]

\section{Technical Extension on Cost Optimization}

\subsubsection{Design Alternative: On-chain storage of operations}

{\bf Use Blockchain for actual log storage}: In our protocol, all operations are uploaded to the Blockchain. An alternative design is to use the Blockchain as the actual data storage. However, Blockchain is ill-suited to be data storage serving online operations. First, Blockchain incurs multiple rounds of confirmations for persisting data, leading to perceivable write latency. Second, when operations access large data records (e.g., multimedia data), storing them directly on Blockchain incurs a high cost. Therefore, in our work, we use Blockchain as a log auditor off the critical path. It records operations at a certain frequency (e.g., every 10 minutes) and only publishes the record hashes\footnote{More precisely, given a key-value record, we can publish to the Blockchain the key hash and the value hash.} to the Blockchain.

\subsubsection{Design: Storage of Historical Operations}
For consistency verification, historical operations need to be persisted. Historical operations are those operations in the previous epochs. They are needed because an operation in the current epoch returns the record written by a historical operation.

A baseline is to maintain all historical operations on chain (e.g., in a smart-contract container). A slightly better approach is to store the ``latest'' snapshot of the records in smart contract. These baselines, however, cause high Blockchain cost as 
they directly persist data on Blockchain and Blockchain is known to be expensive for data storage.

We build a Merkle tree to enable authenticated query processing between the untrusted server and the Blockchain. Briefly, the dataset that historical operations lead to is stored on the untrusted server. The historical dataset is digested by an Merkle tree. The root hash of the Merkle tree is kept in the smart contract on chain. In an epoch, when \texttt{auditLog()} is called, the ContractChecker contract will need to query the historical dataset off-chain (see the example below). When a query of a data key is sent, an ``authentication path'' is constructed by the hash of neighbor nodes along the path from the record to the root in the Merkle tree. This authentication path can be used to prove the membership (or non-membership) of the record in the historical dataset. When \texttt{auditLog()} is completed successfully, all operations in the current epoch are reflected to the off-chain Merkle tree and the on-chain hash root is updated as well.

For instance, consider the operation sequence $w_1(K),w_2(K'),r_3[w_1](K)$ where $w_1w_2(K')$ occurs in Epoch 1 and $r_3[w_1](K)$ occur in Epoch 2. For the Blockchain to assert the consistency of $r_3[w_1]$, it will need to know as of Epoch 2 whether the latest write of data key $K$ is $w_1$. The Blockchain will send out this query to the server and the server who maintains a Merkle tree of the current state (of latest records of all data keys) returns the authentication path for $w_1$, so that its freshness can be verified by the Blockchain.

\subsubsection{Experiments: Blockchain Cost and Storage Capacity}
\begin{figure}[!hbt]
\begin{center}
\subfloat[With varying Gas cost in Ether]{
   \includegraphics[width=0.225\textwidth]{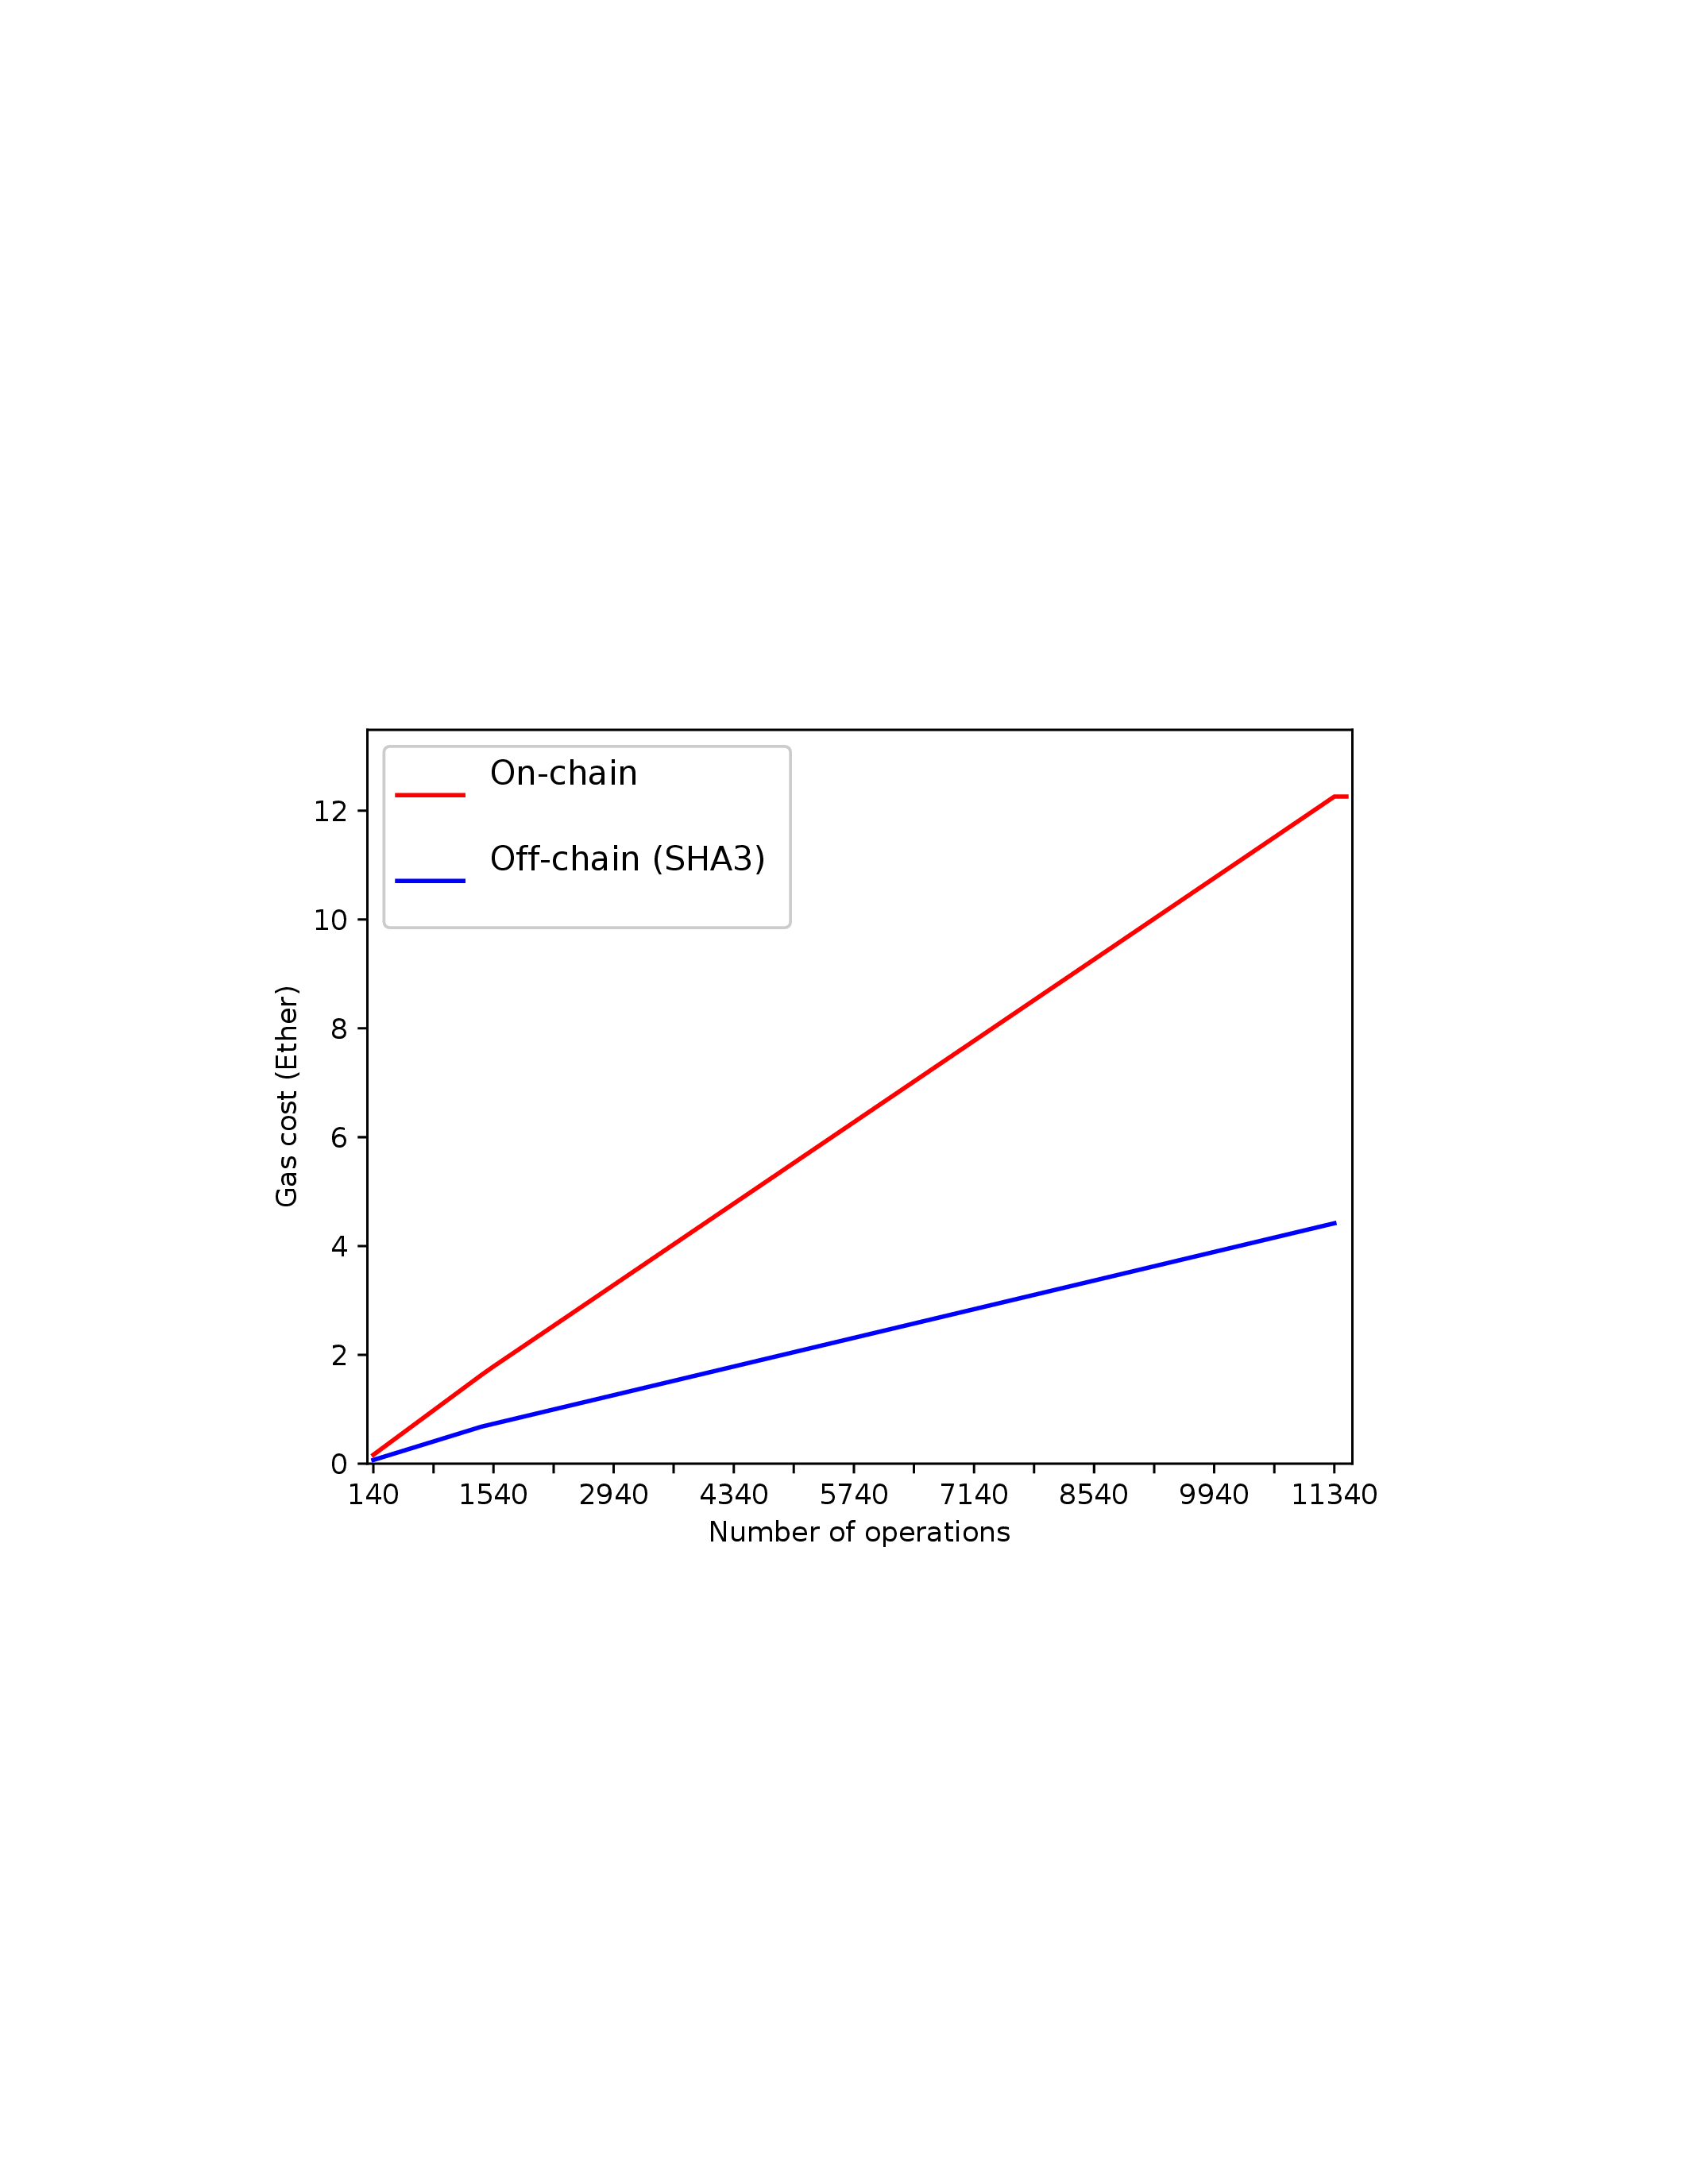}
    \label{exp:capacityether}
}
\subfloat[Storage capacity that can be bought by $\$100$]{
\includegraphics[width=0.225\textwidth]{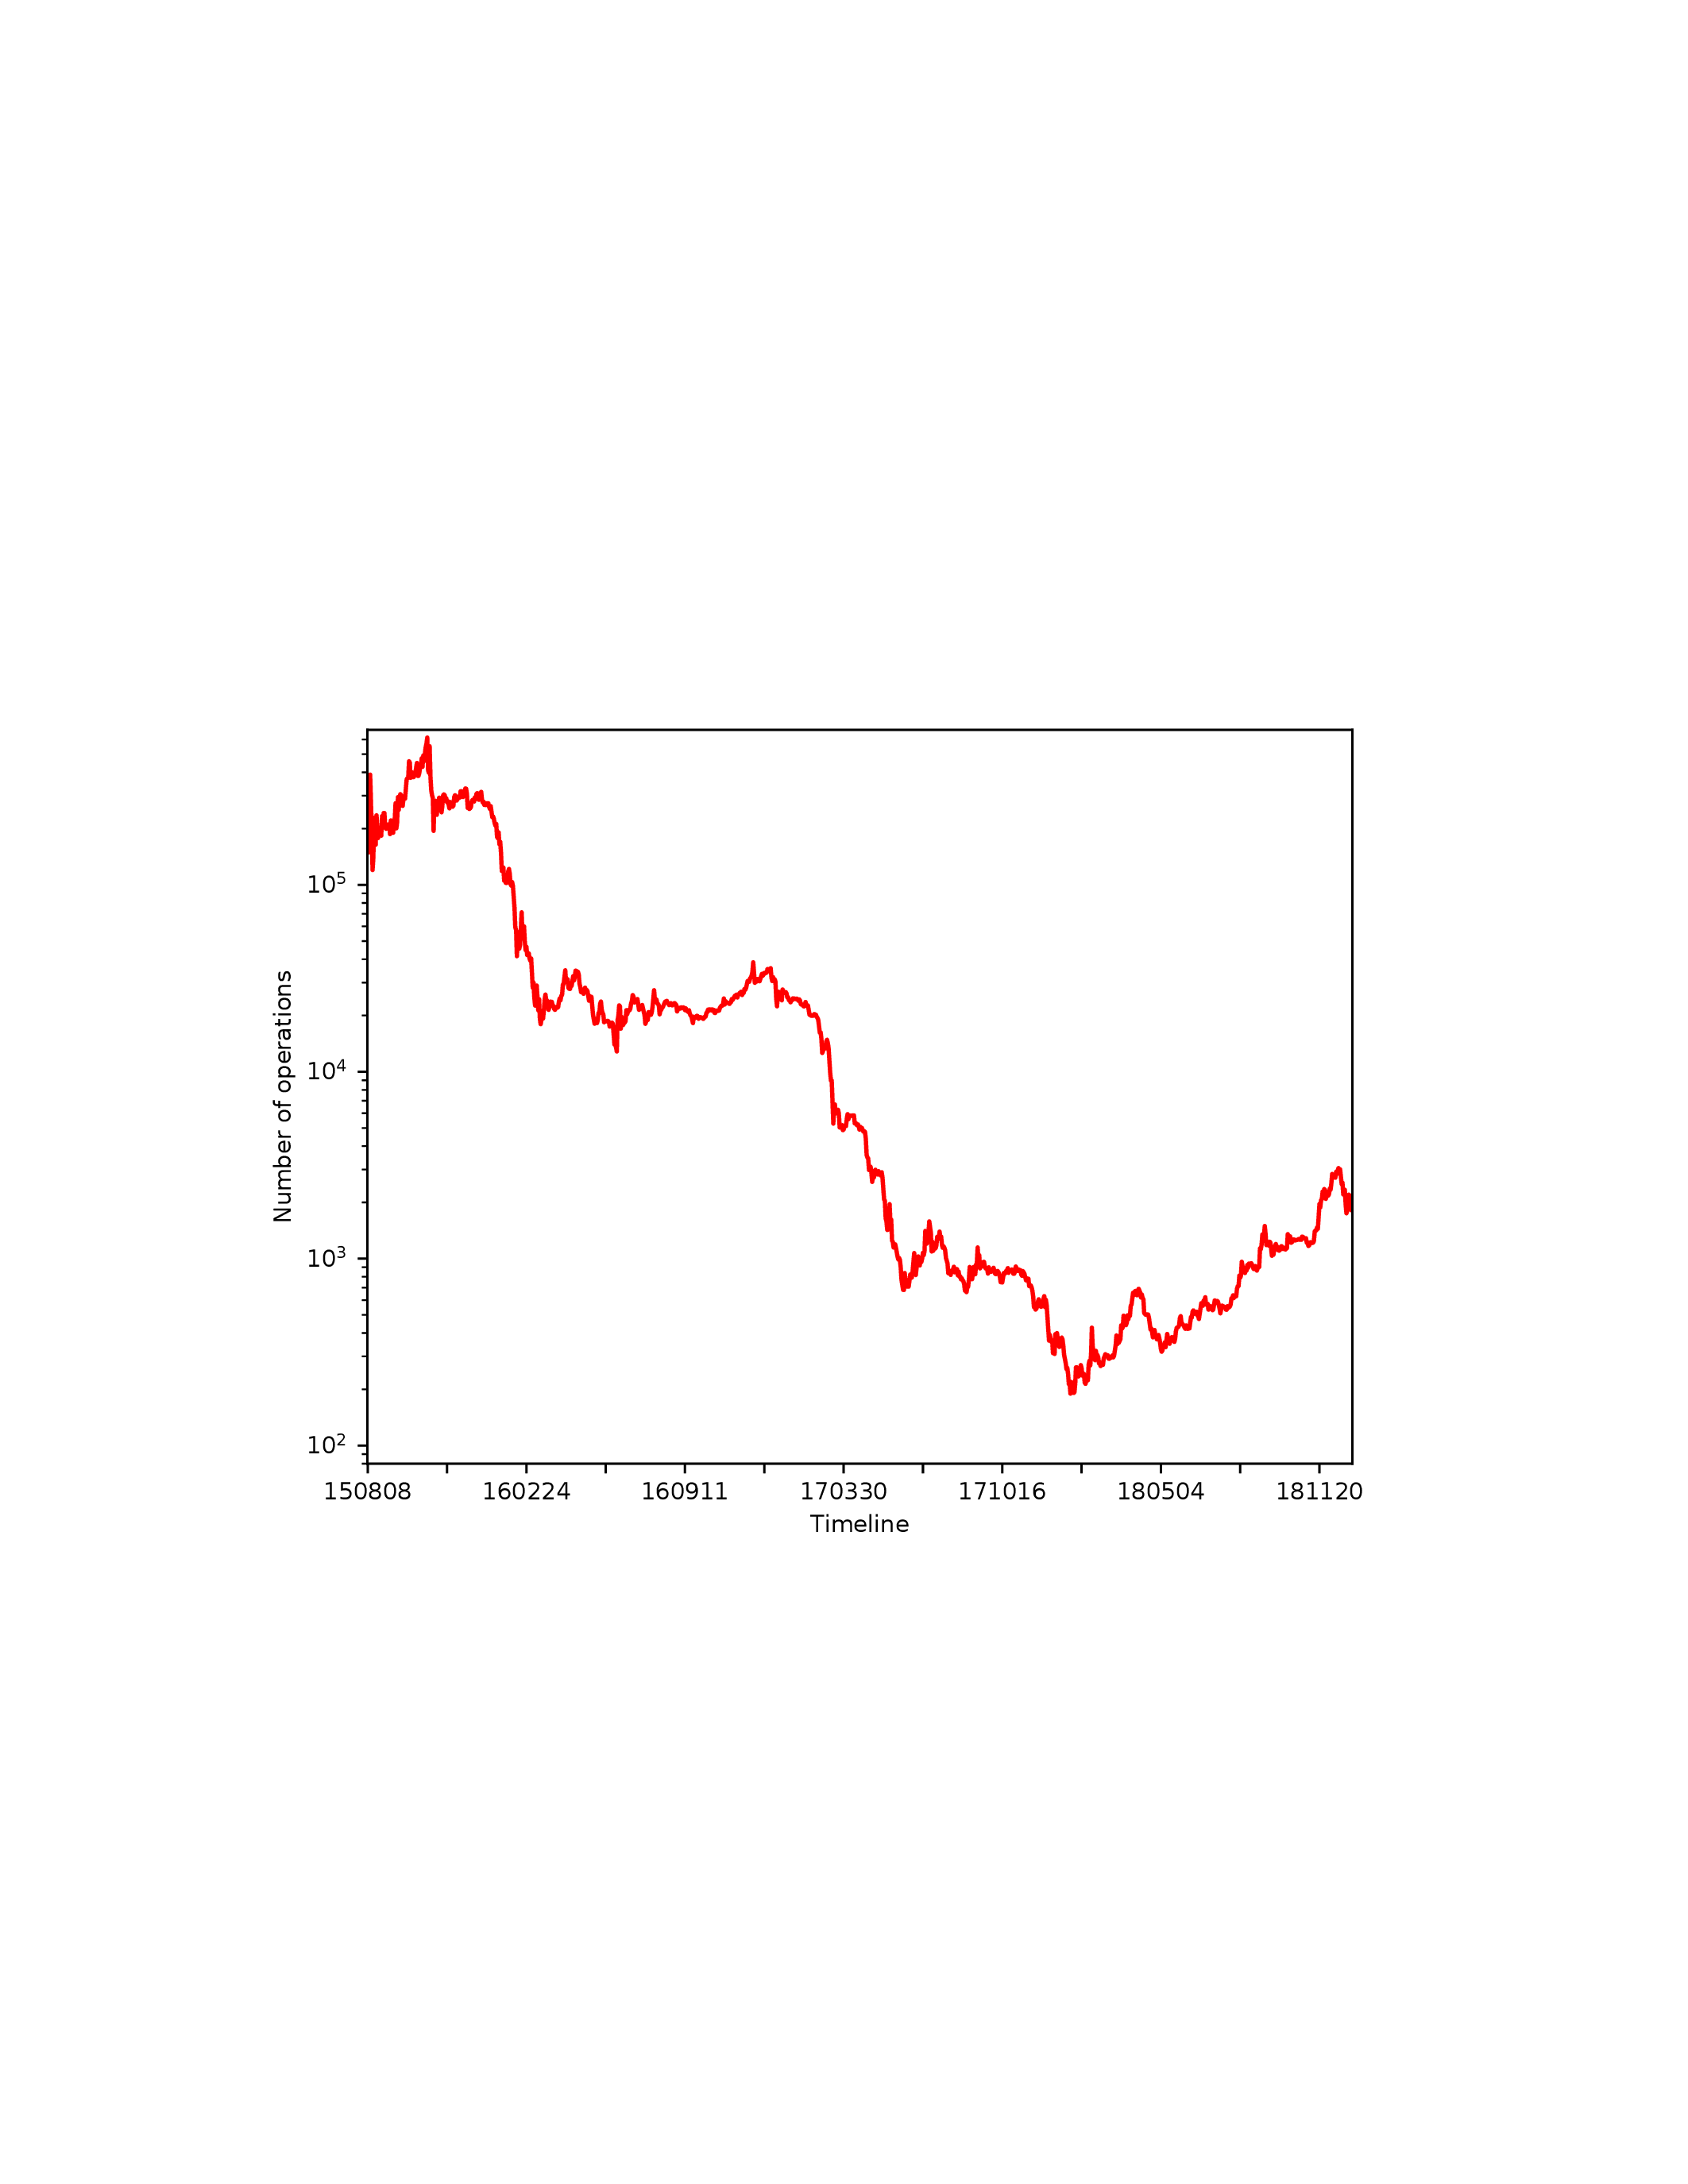}
    \label{exp:capacitydollar}
}
\end{center}
\caption{Storage capacity with Blockchain cost}
\label{exp:capacityether}
\vspace{-0.10in}
\end{figure}

This experiment measures the storage capacity with transactions fee. Given a budget of Ether, ContractChecker's storage capacity is bounded which affects the number of operations the Blockchain can consume and the maximal number of clients it can support. 

In this experiment, we use the YCSB benchmark suit. To adapt YCSB to ContractChecker, we first play and record the YCSB workload trace. We then replay the trace during the experiments. In our experiments, we set an epoch to be one block time (B) and limit 140 operations per epoch (so that Blockchain is not saturated). We set finality delay to be $F\cdot{}B = 6B$.
We drive YCSB workload D (of $95\%$ reads) into ContractChecker. The workload consists of $11340$ operations in total which are evenly distributed among $81$ epochs (with each containing $140$ operations). 
We measure the Gas cost (from the transaction receipt) with the varying number of operations. The result is in Figure~\ref{exp:capacityether}. The Gas cost grows linearly with operation count. For the off-chain placement of historical operations (of both server and client logs), the total Gas is about $4.5$ Ether for $11340$ operations. 

The off-chain placement of historical operations saves $80\%$ of the cost comparing the on-chain placement.
This result shows that transaction fee is cheaper than on-chain storage in Ethereum and the off-chain placement that trades the latter for the former is cost effective.

We also convert the Ether to US dollar and show the dollar cost with ContractChecker storage capacity. Because the price of Ether in US dollar changes over time, we present the ContractChecker storage capacity allowed by $100$ dollars at a different time. The result is illustrated in Figure~\ref{exp:capacitydollar}. It shows that with $100$ dollars, the maximal capability it can buy occurs on Oct. 2015 when the Ether is cheapest. However, as the cryptocurrency price continuously drops in 2018, the ContractChecker will be more cost-effective in US dollar.

\section{Preliminary}

\subsection{Blockchain and Smart Contract}
\label{sec:prel:bkc}

Blockchain is the backend technology in today's cryptocurrencies, such as Bitcoin and Ethereum. This work considers the public Blockchain over the Internet, and do not consider permissioned Blockchains over a private ``consortium'' of players. Physically, a public Blockchain runs in a large-scale peer-to-peer network, where peer nodes, called miners, collectively maintain Blockchain data structures. The P2P network is open-membership in that anyone on the Internet can join. 

We now present the background of Blockchain system from two perspectives that are most relevant to our work: Blockchain as a distributed ledger and Blockchain as a smart-contract execution platform.

{\bf Distributed ledger}: Blockchain is a distributed ledger that stores the history of ``transactions'' for cryptocurrency payment. The Blockchain ledger can be viewed as storage that is publicly readable and is writable by decentralized authorities namely miners. In particular, writing a transaction to Blockchain goes through the following pipeline: 1) The transaction is broadcast to all miners, pending in their memory pools. 2) Pending transactions are selected (e.g., by transaction fee) to be validated based on some prescribed rules (e.g., no double spending transactions). 3) All Blockchain nodes run a consensus protocol to decide which valid transactions are to be included next in the Blockchain ledger. Following this pipeline, every ``block time'' $B$, the Blockchain is expected to produce a new block of accepted transactions. 

Writing a transaction to a Blockchain is {\it asynchronous} in the sense that it takes a long delay to confirm if the transaction is finally included in Blockchain. More precisely, only after there are $F$ blocks produced after the transaction, the transaction is considered finalized on the Blockchain. That is, it will be hard to change the transaction state on Blockchain. Writing a transaction to a Blockchain can {\it fail} in the sense that the Blockchain can drop valid transactions in some circumstances. For example, when the transaction throughput is larger than Blockchain's throughput limits\footnote{Public Blockchains are considered as low-throughput systems that accept just tens of transactions per second.} or transaction fee is too low,  Blockchain will drop transactions. In other words, Blockchain may have low write availability in the above conditions.

{\bf Contract execution}: Blockchain is also an execution platform for \emph{smart contact}. Smart contract is a program that can be executed in modern Blockchains, such as Ethereum and that is originally proposed to support financial applications over Blockchain. To execute a smart contract, the contract author writes a program, compiles it to bytecode and deploys it to the Blockchain by encoding the compiled bytecode in a special Blockchain transaction. Once the contract is deployed on all Blockchain miners, a party off-chain will be able to trigger the contract execution by sending another transaction encoding the runtime arguments. Internally, a smart contract is executed as a replicated state machine on Blockchain miners. That is, the execution instances are spawn and replicated across all miner nodes. Running a contract function is a state transition to the Blockchain where the begin and end contract states are encoded in two blocks in Blockchain and all miners running the contract race to include the execution result in the end block.

In public Blockchain, a fundamental security assumption is that the majority of miners are honest nodes in the sense that they execute the Blockchain software by honestly following the prescribed protocol. In the case of 51\% attacks where the majority of miners are malicious, many Blockchain security properties are broken. In practice, compromising $51\%$ of miners in a large-scale Blockchain network is extremely hard and we believe this is reasonable to assume an honest majority. There are more sophisticated attacks, such as selfish mining~\cite{DBLP:conf/fc/EyalS14}, that require only $33\%$ malicious miners, but they never happen in practice and we do not consider them in this paper.

{\bf Blockchain forks}: This work focuses on practical forks in real-world public Blockchains, and excludes theoretic Blockchain forks (due to $51\%$ attacks, selfish mining, etc.). There are two types of Blockchain forks: a transient fork among miners on recently found blocks, and a permanent fork among different Blockchain networks. 
The transient fork (the former) in a public Blockchain is eventually resolved after the finality delay when all miners reach consensus on one fork while other forks are orphaned. The permanent fork (the latter) is caused by the ``hard fork'' in Blockchain software updates (e.g., the case of bitcoin and bitcoin cash), launching an Alt coin (i.e., by running Blockchain software among a group of friends), etc. It is found common in practice. 

{\bf Blockchain cost} includes the fee to send a transaction and the cost of running smart-contracts. The higher a transaction fee is, the more likely the transaction will be included in the next block. For the smart-contract, any contract on chain needs to be associated with a cost budget, called ``Gas'', which bounds the execution time of the contract and is a mechanism for the defense of DoS (denial of service) attacks.

\section{Misc. of the system}

\subsubsection{ContractChecker Epoch Configuration}
\label{sec:settinge}

ContractChecker runs in epochs. The duration of an epoch $E$ can be configured in practice to respect various application-level requirements. In general, a large $E$ is preferred when 1) the application can afford longer delay in consistency assertion, 2) the clients tend to be available in a longer time period after their interaction with the cloud server, 3) there are more clients producing more attestations transactions in an epoch.

While the first two requirements are applications specific, we present a model for the third requirement. For simplicity, we consider epoch duration $E$ is set to be multiple of the block time $B$, namely $E=e\times{}B$. 
The value of $e$ must be set large enough to avoid the attestation transactions saturate the Blockchain. For instance, suppose there are $N=30$ clients and a Block can only store 20 transactions. Setting $e=1$ may saturate the Blockchain limited throughput as every block time, the protocol produces $30+1$ transactions which are above what the Blockchain can ingest (i.e., $20$ transaction per block). In this case, it is advised to configure $e\geq{2}$, such that the $31$ attestation transactions produced in each epoch can be amortized to at least two blocks.

\subsubsection{Identity Management}
\label{sec:identity}
In ContractChecker, both clients and the server are registered in the sense that their public keys are known by the contract code. The public keys are used to verify the log attestations from clients and the server. The log verification is necessary to prevent anyone from injecting arbitrary operations in the log which can easily obstruct the consistency assertion.

To set up the public keys, we assume a secure key-distribution channel exists. Clients can dynamically join and register; we assume an external trusted identity provider in place who assists the user authentication and sends the new public keys to the smart contract.

The clients and server can reuse the public key pair in their Blockchain wallets for ContractChecker operations. In this work, we assume the secret keys are securely managed by clients and server offline. With securely managed keys, a variety of attacks, e.g., clients and server impersonation, are prevented.
